# Supplementary material for: A universal low-temperature fluctuation of unconventional superconductivity revealed: Smoking gun favors Galilean bosonic superfluidity
Source: arXiv:2402.08730 ancillary file (2026-09-28)
Supplement: Supplementary file 1 [file Appendix.pdf]

## Appendix

In this appendix we rigorously derive the superfluid component of the dynamic current-current response function, identifying it with the true condensate divided by the bare mass, for a general interacting bosonic system. We then demonstrate the particle-hole excitation nature of the linear dispersion, and use this dispersion in appropriate thermal ensemble to identify the leading order depletion of the superfluid density with temperature to be  $\propto T^3$ . We also show that introducing weak impurities perturbatively to leading order increases this depletion to be  $\propto T$ . In addition, we provide a no-go theorem preventing the use of an ensemble of ‘sound’ waves to describe the normal fluid, and then we showcase the inconsistency resulting from such a construction. Finally, we describe the details for the extraction and fitting procedures used to obtain the data collapse illustrated in the main text, and further exhibit the doping-independence of the universal  $T^3$  depletion in a YBCO example.

Section IA defines the eigenbasis of a general interacting bosonic system via canonical transformation, and IB identifies important physical properties preserved in this transformation for each particle. In section II we demonstrate the linear dispersion of the particle-hole excitation in a straightforward particle-conserving version of the Bogoliubov low-energy effective model, identifying the ‘sound’ mode excitation operator of that system as a systematic approximation to the true particle-hole excitation operator defined in the canonical transformation of section I. Section IIIA reviews the operator form of the continuity equation and section IIIB reviews the  $f$ -sum rule in the context of the canonically-transformed eigenbasis defined in section I. We then derive a rule of partial sums satisfied by the dynamic response for each momentum in section IIIC. In section IVA we define the dressed current operator, and in IVB prove that it maps to the bare current operator in the long-wavelength limit. We are then able to derive the superfluid component of the dynamic response using the dressed current operator in section IVC and show that it is directly proportional to the true condensate defined in section IA. We then use the linear dispersion of the particle-hole excitations identified in section II to study the thermodynamic statistics of the true condensate density as an estimate in the grand canonical ensemble in section VA and rigorously derived in the canonical ensemble in section VB. Section VI presents a no-go theorem that forbids an ensemble of curl-less waves, such as phonons, from representing the normal fluid response, and section VII illustrates an inconsistency that results from such an ensemble. In section VIII we study the leading order perturbative contribution to the depletion of the superfluid density with temperature in the presence of weak impurities. In section IX we describe the fitting method and plotting procedure used to generate Figure 1 in the main text. Finally, in section X we show that the universal  $T^3$  superfluid depletion is also independent of doping in YBCO.

### I. HAMILTONIAN AND HILBERT SPACE

#### A. Definition and diagonalization via canonical transformation

Consider a generic  $N$ -particle interacting bosonic system on a lattice with  $\mathcal{V}$  sites that hosts standard superfluidity, described by a Hamiltonian  $H[\{a_{\mathbf{R}}^\dagger\}]$  represented by local second-quantized creation operators  $a_{\mathbf{R}}^\dagger$  with corresponding Hamiltonian

$$H = \sum_{\mathbf{R}\mathbf{R}'} t_{\mathbf{R}\mathbf{R}'} a_{\mathbf{R}}^\dagger a_{\mathbf{R}'} + \frac{1}{2} \sum_{\mathbf{R}-\mathbf{R}'} V_{\mathbf{R}-\mathbf{R}'} a_{\mathbf{R}}^\dagger a_{\mathbf{R}'}^\dagger a_{\mathbf{R}'} a_{\mathbf{R}}, \quad (1)$$

where  $t_{\mathbf{R}\mathbf{R}'}^* = t_{\mathbf{R}'\mathbf{R}}$  are the hopping parameters, and  $V_{\mathbf{R}-\mathbf{R}'}$  is any generic translation-symmetric density-density interaction (for example, the Coulomb potential or the Hubbard interaction  $U$ ). Represented via second-quantized creation operators of momentum  $a_{\mathbf{k}}^\dagger$ , the Hamiltonian becomes

$$H = \sum_{\mathbf{k}} \epsilon_{\mathbf{k}} a_{\mathbf{k}}^\dagger a_{\mathbf{k}} + \frac{1}{2\mathcal{V}} \sum_{\mathbf{k}\mathbf{p}\mathbf{q}} V(\mathbf{q}) a_{\mathbf{k}+\mathbf{q}}^\dagger a_{\mathbf{p}-\mathbf{q}}^\dagger a_{\mathbf{p}} a_{\mathbf{k}}, \quad (2)$$

where  $V(\mathbf{q})$  can only be a function of the internal momentum  $\mathbf{q}$ .

Eq.(2) can always be brought to a diagonal truncating form

$$\begin{aligned} H_{\text{diag}}[\{\tilde{a}_{\mathbf{k}}^\dagger\}] &\equiv H[\{a_{\mathbf{k}}^\dagger\}] \\ &= \sum_{\mathbf{k}_1} \epsilon_{\mathbf{k}_1} \tilde{a}_{\mathbf{k}_1}^\dagger \tilde{a}_{\mathbf{k}_1} + \frac{1}{2!} \sum_{\mathbf{k}_1\mathbf{k}_2} \epsilon_{\mathbf{k}_1\mathbf{k}_2} \tilde{a}_{\mathbf{k}_1}^\dagger \tilde{a}_{\mathbf{k}_2}^\dagger \tilde{a}_{\mathbf{k}_2} \tilde{a}_{\mathbf{k}_1} \\ &+ \frac{1}{3!} \sum_{\mathbf{k}_1\mathbf{k}_2\mathbf{k}_3} \epsilon_{\mathbf{k}_1\mathbf{k}_2\mathbf{k}_3} \tilde{a}_{\mathbf{k}_1}^\dagger \tilde{a}_{\mathbf{k}_2}^\dagger \tilde{a}_{\mathbf{k}_3}^\dagger \tilde{a}_{\mathbf{k}_3} \tilde{a}_{\mathbf{k}_2} \tilde{a}_{\mathbf{k}_1} + \dots \\ &+ \frac{1}{N!} \sum_{\mathbf{k}_1 \dots \mathbf{k}_N} \epsilon_{\mathbf{k}_1 \dots \mathbf{k}_N} \tilde{a}_{\mathbf{k}_1}^\dagger \dots \tilde{a}_{\mathbf{k}_N}^\dagger \tilde{a}_{\mathbf{k}_N} \dots \tilde{a}_{\mathbf{k}_1}, \end{aligned} \quad (3)$$

using the corresponding one-body eigenoperators,

$$\tilde{a}_{\mathbf{k}}^\dagger = U^\dagger a_{\mathbf{k}}^\dagger U, \quad (4)$$

transformed from the ‘bare’ creation operators  $a_{\mathbf{k}}^\dagger$  via a unitary operator  $U$ .

Owing to the diagonal structure of  $H_{\text{diag}}$  and the standard bosonic commutation,

$$[\tilde{a}_{\mathbf{k}}, \tilde{a}_{\mathbf{p}}^\dagger] = \delta_{\mathbf{k}\mathbf{p}} \quad (5)$$

$$[\tilde{a}_{\mathbf{k}}, \tilde{a}_{\mathbf{p}}] = 0, \quad (6)$$

each  $N$ -body eigenstate  $|\{N_{\mathbf{k}}\}\rangle$  is constructed by unique repeated application of the set of eigenoperators  $\{\tilde{a}_{\mathbf{k}}^\dagger\}$  to the zero particle vacuum  $|0\rangle$ . These states form a complete orthonormal  $N$ -body basis and take the form of direct products,

$$|\{N_{\mathbf{k}}\}\rangle \equiv \prod_{\mathbf{k}} \frac{(\tilde{a}_{\mathbf{k}}^\dagger)^{N_{\mathbf{k}}}}{\sqrt{N_{\mathbf{k}}!}} |0\rangle \Big|_{\sum_{\mathbf{k}} N_{\mathbf{k}} = N}, \quad (7)$$

as all the many-body quantum fluctuations are fully absorbed in  $\tilde{a}_{\mathbf{k}}^\dagger$ .

For systems where the kinetic energy dominates over the interaction  $V$ , such as those of interest in this study, the ground state is simply

$$|\Omega\rangle \equiv \frac{(\tilde{a}_0^\dagger)^N}{\sqrt{N!}} |0\rangle, \quad (8)$$

with all  $N$  particles having lowest kinetic energy at zero momentum. Correspondingly, the ground state is a ‘true’ Bose-Einstein condensate containing all  $N$  particles

$$\langle \Omega | \hat{N}_0 | \Omega \rangle \equiv \langle \Omega | \tilde{a}_0^\dagger \tilde{a}_0 | \Omega \rangle = N. \quad (9)$$

## B. Properties preserved in the canonical transformation

The details of the dressing of each particle due to the interaction are complicated. However, the essential properties of number  $N$ , mass  $\hat{M}$ , and momentum  $\hat{P}$  are preserved under this transformation in general, which we now derive below.

A helpful property of the unitary transformation identified in Eq.(4) of Section I A is that it takes identical form when represented by the dressed operators  $\{\tilde{a}_{\mathbf{k}}^\dagger\}$  as when it is represented by the bare operators  $\{a_{\mathbf{k}}^\dagger\}$

$$\begin{aligned} \hat{U}[\{\tilde{a}_{\mathbf{k}}\}] &= \hat{U}[\{\hat{U}^\dagger a_{\mathbf{k}} \hat{U}\}] \\ &= \hat{U}^\dagger (\hat{U}[\{a_{\mathbf{k}}\}]) \hat{U} \\ &= \hat{U}[\{a_{\mathbf{k}}\}], \end{aligned} \quad (10)$$

where the second equality can be seen by expressing  $\hat{U}$  in an operator expansion of  $\{\tilde{a}_{\mathbf{k}}\}$  and using the property of unitarity  $\hat{U}\hat{U}^\dagger = 1$ , and the third equality holds since  $\hat{U}$  trivially commutes with itself.

The Hamiltonian in Eq.(2) preserves particle number and therefore commutes with the total particle number operator

$$[N, H] = 0. \quad (11)$$

Since the unitary transformation  $\hat{U}$  preserves the symmetries of the Hamiltonian  $H$ ,  $N$  must also commute with it

$$[N, \hat{U}] = 0. \quad (12)$$

Starting with the sum over dressed density operators,

$$\begin{aligned} \sum_{\mathbf{k}} \tilde{a}_{\mathbf{k}}^\dagger \tilde{a}_{\mathbf{k}} &= \sum_{\mathbf{k}} \hat{U}^\dagger a_{\mathbf{k}}^\dagger \hat{U} \hat{U}^\dagger a_{\mathbf{k}} \hat{U} \\ &= \hat{U}^\dagger \left( \sum_{\mathbf{k}} a_{\mathbf{k}}^\dagger a_{\mathbf{k}} \right) \hat{U} \\ &= N, \end{aligned} \quad (13)$$

we find that it is simply the total number operator  $N$ .

Given that each bare particle has the same mass  $m$ ,

$$\begin{aligned}\hat{M} &= \sum_{\mathbf{k}} m a_{\mathbf{k}}^{\dagger} a_{\mathbf{k}} \\ &= m \left( \sum_{\mathbf{k}} a_{\mathbf{k}}^{\dagger} a_{\mathbf{k}} \right) \\ &= mN \\ &= m \sum_{\mathbf{k}} \tilde{a}_{\mathbf{k}}^{\dagger} \tilde{a}_{\mathbf{k}}\end{aligned}\tag{14}$$

each dressed particle retains mass  $m$  as well, where we used the above representation derived for  $N$ .

Finally, since the Hamiltonian conserves total momentum  $\hat{P} = \sum_{\mathbf{k}} \hbar \mathbf{k} a_{\mathbf{k}}^{\dagger} a_{\mathbf{k}}$ , the total momentum operator commutes yet again with both  $H$  and the symmetry preserving  $\hat{U}$ ,

$$[\hat{P}, \hat{U}] = 0.\tag{15}$$

Therefore, a derivation identical to that for  $N$  above holds for the total momentum operator,

$$\hat{P} = \sum_{\mathbf{k}} \hbar \mathbf{k} \tilde{a}_{\mathbf{k}}^{\dagger} \tilde{a}_{\mathbf{k}},\tag{16}$$

proving that each dressed particle carries the same (kinematic) momentum as its corresponding bare particle. Note that, as a corollary of Eqs.(14,16), the dressed particle also retains the average bare kinematic velocity

$$\frac{1}{N} \sum_{\mathbf{k}} \frac{\hbar \mathbf{k}}{m} a_{\mathbf{k}}^{\dagger} a_{\mathbf{k}} = \frac{1}{N} \sum_{\mathbf{k}} \frac{\hbar \mathbf{k}}{m} \tilde{a}_{\mathbf{k}}^{\dagger} \tilde{a}_{\mathbf{k}},\tag{17}$$

as denoted in the main text.

## II. DEMONSTRATION OF THE LINEAR DISPERSION OF ‘SOUND’ DUE TO PARTICLE-HOLE EXCITATIONS

In this section we identify the linear dispersion of ‘sound’ (i.e. quanta of longitudinal waves)<sup>1</sup> and its equivalent description as particle-hole excitations via a demonstration of the eigensolution for the low-energy Hamiltonian in an approximation that preserves particle number. In particular we show the resulting linear dispersion and the form of the particle-hole excitations, which provide a leading order approximation to the particle-hole excitations of the true diagonalized Hamiltonian.

We begin by representing the low-energy Hamiltonian, in the presence of macroscopic occupation in the lowest one-body state of the non-interacting eigenbasis  $a_0^{\dagger} a_0 \equiv N_0 \gg 1$ , by particle-hole excitation operators that preserve particle number

$$\alpha_{\mathbf{k}}^{\dagger} \equiv \frac{a_{\mathbf{k}}^{\dagger} a_0}{\sqrt{N_0 + 1}} \quad \forall \mathbf{k} \neq 0\tag{18}$$

$$\alpha_{\mathbf{k}} \equiv \frac{a_0^{\dagger} a_{\mathbf{k}}}{\sqrt{N_0 + 1}} \quad \forall \mathbf{k} \neq 0.\tag{19}$$

Notice the particle-hole excitation nature of the operators in Eqs.(18,19) and their close analogy to the excitation operators in linear spin wave theory<sup>2</sup>.

We can now represent  $H$  using the real-particle conserving operators defined in Eqs.(18,19). Separating the total number operator  $N$  into a bare condensate part and the rest,

$$N = \sum_{\mathbf{k}} a_{\mathbf{k}}^{\dagger} a_{\mathbf{k}} = a_0^{\dagger} a_0 + \sum_{\mathbf{k} \neq 0} a_{\mathbf{k}}^{\dagger} a_{\mathbf{k}},\tag{20}$$

we can rewrite the kinetic energy in Eq.(2),

$$\sum_{\mathbf{k}} \epsilon_{\mathbf{k}} a_{\mathbf{k}}^{\dagger} a_{\mathbf{k}} = \sum_{\mathbf{k} \neq 0} (\epsilon_{\mathbf{k}} - \epsilon_0) \alpha_{\mathbf{k}}^{\dagger} \alpha_{\mathbf{k}} + \epsilon_0 N,\tag{21}$$

into a particle-hole excitation form up to a term  $\epsilon_0 N$  that commutes with  $H$ .

For the interaction in Eq.(2), we use an example that is  $\mathbf{q}$ -independent  $V(\mathbf{q}) = V$ . Starting similarly to the standard approach by using the large condensate  $N_0 \gg 1$  to include only those terms up to bilinear in  $\mathbf{k} \neq \mathbf{0}$ ,

$$\begin{aligned} \frac{V}{\mathcal{V}} \sum_{\mathbf{k}\mathbf{p}\mathbf{q}} a_{\mathbf{k}+\mathbf{q}}^\dagger a_{\mathbf{p}-\mathbf{q}}^\dagger a_{\mathbf{p}} a_{\mathbf{k}} &= \frac{V}{\mathcal{V}} a_0^\dagger a_0^\dagger a_0 a_0 + \frac{V}{2\mathcal{V}} \sum_{\mathbf{k} \neq \mathbf{0}} (4a_{\mathbf{k}}^\dagger a_0^\dagger a_0 a_{\mathbf{k}} + a_{\mathbf{k}}^\dagger a_{-\mathbf{k}}^\dagger a_0 a_0 + a_0^\dagger a_0^\dagger a_{\mathbf{k}} a_{-\mathbf{k}}) + H_{\text{fluc}} \\ &\approx V n_0 (N_0 - 1) + \frac{V n_0}{2} \sum_{\mathbf{k} \neq \mathbf{0}} (4\alpha_{\mathbf{k}}^\dagger \alpha_{\mathbf{k}} + \alpha_{\mathbf{k}}^\dagger \alpha_{-\mathbf{k}}^\dagger + \alpha_{\mathbf{k}} \alpha_{-\mathbf{k}}), \end{aligned} \quad (22)$$

where  $n_0 = N_0/\mathcal{V}$ , and  $H_{\text{fluc}}$  are the remaining neglected terms from the bare interaction. The standard approach results in generally particle-non-conserving terms such as  $a_{\mathbf{k}}^\dagger a_{-\mathbf{k}}^\dagger$  in the interaction. In contrast, all of our interaction terms in Eq.(22) are inherently particle-conserving and ensure that every many-body state remains strictly in the  $N$ -particle sector.

Combining Eqs.(21,22) the Hamiltonian becomes

$$H \equiv \Xi_0 + H_{\text{ex}} + H_{\text{fluc}} \quad (23)$$

$$H_{\text{ex}} = \sum_{\mathbf{k} \neq \mathbf{0}} \left( (\epsilon_{\mathbf{k}} - \epsilon_0 + 2V n_0) \alpha_{\mathbf{k}}^\dagger \alpha_{\mathbf{k}} + \frac{V n_0}{2} (\alpha_{\mathbf{k}}^\dagger \alpha_{-\mathbf{k}}^\dagger + \alpha_{\mathbf{k}} \alpha_{-\mathbf{k}}) \right), \quad (24)$$

where  $\Xi_0$  is the  $N$ -body ground state energy.

After diagonalization, the resulting solution is

$$H_{\text{ex}} = \sum_{\mathbf{k} \neq \mathbf{0}} \Omega_{\mathbf{k}} \tilde{\alpha}_{\mathbf{k}}^\dagger \tilde{\alpha}_{\mathbf{k}} \quad (25)$$

$$\Omega_{\mathbf{k}} = \sqrt{\epsilon_{\mathbf{k}}(2V n_0 + \epsilon_{\mathbf{k}})} \quad (26)$$

$$\tilde{\alpha}_{\mathbf{k}}^\dagger = c_{\mathbf{k}} \alpha_{\mathbf{k}}^\dagger + d_{\mathbf{k}} \alpha_{-\mathbf{k}} \quad (27)$$

$$c_{\mathbf{k}} = \sqrt{\frac{\epsilon_{\mathbf{k}} + V n_0 + \Omega_{\mathbf{k}}}{2\Omega_{\mathbf{k}}}} \quad (28)$$

$$d_{\mathbf{k}} = \sqrt{\frac{\epsilon_{\mathbf{k}} + V n_0 - \Omega_{\mathbf{k}}}{2\Omega_{\mathbf{k}}}}. \quad (29)$$

The solution in Eqs.(26-29) is completely different from, for example, the traditional Bogoliubov quasiparticle solution, since our operators  $\alpha_{\mathbf{k}}$  are particle-conserving.

Importantly, we can see that these particle-hole excitations  $\tilde{\alpha}_{\mathbf{k}}^\dagger$  follow a linear dispersion in Eq.(26), and that the excitations generated by  $\alpha_{\mathbf{k}}^\dagger$  are not conserved in Eq.(24) even though the underlying particles are conserved. These results support the interpretation of these ‘sound’ modes  $\tilde{\alpha}_{\mathbf{k}}^\dagger$  as the leading order contribution to the dressed particle-hole excitation operator,  $\tilde{\alpha}_{\mathbf{k}} = \tilde{a}_{\mathbf{k}}^\dagger \tilde{a}_{\mathbf{k}}$ , defined via the dressed particles in Eq.(4) and indicate that the dispersion for the dressed particle-hole operators is linear at low energy.

### III. STATE-INDEPENDENT RESPONSE

#### A. Continuity equation in general operator form

We now review the continuity equation and the corresponding  $f$ -sum rule for the current-current response in a very general operator formulation. The results of this section will simplify the study of the dressed current in the following section.

In the standard literature<sup>3</sup>, the polarization operator

$$\Pi = \sum_{\mathbf{R}} \mathbf{R} a_{\mathbf{R}}^\dagger a_{\mathbf{R}}, \quad (30)$$

where  $\mathbf{R}$  is the position of the particles, can be used to derive the current operator via its time derivative,

$$\mathbf{J} = \frac{d\Pi}{dt} = \frac{1}{i\hbar} [\Pi, H] = \frac{1}{i\hbar} \sum_{\mathbf{R}\mathbf{R}'} \delta_{\mathbf{R}\mathbf{R}'} t_{\mathbf{R}\mathbf{R}'} a_{\mathbf{R}}^\dagger a_{\mathbf{R}'}, \quad (31)$$

where we have used the Hamiltonian in Eq.(1), and  $\delta_{\mathbf{R}\mathbf{R}'} = \mathbf{R} - \mathbf{R}'$  is the vector difference between sites  $\mathbf{R}$  and  $\mathbf{R}'$ . Notice that the interaction in Eq.(1) only depends on the density and therefore commutes with the polarization operator.

By defining a semi-local bond current at  $\bar{\mathbf{R}} \equiv (\mathbf{R} + \mathbf{R}')/2$ ,

$$\mathbf{J}_{\bar{\mathbf{R}}} = \frac{1}{i\hbar} \delta_{\mathbf{R}\mathbf{R}'} (t_{\mathbf{R}\mathbf{R}'} a_{\mathbf{R}}^\dagger a_{\mathbf{R}'} - t_{\mathbf{R}'\mathbf{R}} a_{\mathbf{R}'}^\dagger a_{\mathbf{R}}), \quad (32)$$

We can obtain a continuity equation on the lattice

$$\frac{dn_{\mathbf{R}}}{dt} = - \sum_{\mathbf{R}'} \frac{\delta_{\mathbf{R}'\mathbf{R}}}{|\delta_{\mathbf{R}'\mathbf{R}}|^2} \cdot \mathbf{J}_{\bar{\mathbf{R}}}, \quad (33)$$

where  $n_{\mathbf{R}}$  is the local density operator

$$n_{\mathbf{R}} = a_{\mathbf{R}}^\dagger a_{\mathbf{R}}. \quad (34)$$

The continuity equation in Eq.(33) can be further checked via the Heisenberg equation of motion

$$\frac{dn_{\mathbf{R}}}{dt} = \frac{1}{i\hbar} [n_{\mathbf{R}}, H] = \frac{1}{i\hbar} \sum_{\mathbf{R}'} (t_{\mathbf{R}\mathbf{R}'} a_{\mathbf{R}}^\dagger a_{\mathbf{R}'} - t_{\mathbf{R}'\mathbf{R}} a_{\mathbf{R}'}^\dagger a_{\mathbf{R}}) = - \sum_{\mathbf{R}'} \frac{\delta_{\mathbf{R}'\mathbf{R}}}{|\delta_{\mathbf{R}'\mathbf{R}}|^2} \cdot \mathbf{J}_{\bar{\mathbf{R}}} \quad (35)$$

verifying that the bond current at  $(\mathbf{R} + \mathbf{R}')/2$  properly conserves particle number on the lattice. Note in particular that, in the long-wavelength limit, Eq.(33) reduces to the standard form of continuity equation

$$\frac{dn(\mathbf{R})}{dt} + \nabla \cdot \mathbf{J}(\mathbf{R}) = 0. \quad (36)$$

Below, it will be most convenient to use a momentum representation. From the Fourier transform of the bond current operator,

$$\mathbf{J}_{\mathbf{q}} \equiv \frac{1}{\mathcal{V}} \sum_{\mathbf{R}} \mathbf{J}_{\bar{\mathbf{R}}} e^{i\mathbf{q} \cdot \bar{\mathbf{R}}}, \quad (37)$$

the current reduces to

$$\mathbf{J}_{\mathbf{q}} = \frac{1}{\hbar \mathcal{V}} \sum_{\mathbf{k}} (\nabla_{\mathbf{k}'} \varepsilon_{\mathbf{k}'} )|_{\mathbf{k}'=\mathbf{k}+\frac{\mathbf{q}}{2}} a_{\mathbf{k}+\frac{\mathbf{q}}{2}}^\dagger a_{\mathbf{k}}, \quad (38)$$

where  $\varepsilon_{\mathbf{k}} = \sum_{\mathbf{R}'} t_{\mathbf{R}\mathbf{R}'} e^{i\mathbf{k} \cdot (\mathbf{R}' - \mathbf{R})}$  is the bare dispersion.

From the Fourier transform of Eq. (34)

$$n_{\mathbf{q}} = \frac{1}{\mathcal{V}} \sum_{\mathbf{k}} a_{\mathbf{k}+\mathbf{q}}^\dagger a_{\mathbf{k}}, \quad (39)$$

the continuity equation is simply

$$\begin{aligned} \frac{dn_{\mathbf{q}}}{dt} &= \frac{1}{i\hbar} \left[ n_{\mathbf{q}}, \sum_{\mathbf{k}} \varepsilon_{\mathbf{k}} a_{\mathbf{k}}^\dagger a_{\mathbf{k}} \right] \\ &= \frac{1}{\mathcal{V}} \frac{1}{i\hbar} \sum_{\mathbf{k}} a_{\mathbf{k}+\mathbf{q}}^\dagger a_{\mathbf{k}} (\varepsilon_{\mathbf{k}} - \varepsilon_{\mathbf{k}+\mathbf{q}}). \end{aligned} \quad (40)$$

The continuity equation in Eq.(40) takes a particularly simple form when represented by  $\mathbf{J}_{\mathbf{q}}$  from Eq.(38)

$$\frac{dn_{\mathbf{q}}}{dt} - i\mathbf{q} \cdot \mathbf{J}_{\mathbf{q}} = \frac{i}{\hbar \mathcal{V}} \sum_{\mathbf{k}} \left\{ (\varepsilon_{\mathbf{k}+\mathbf{q}} - \varepsilon_{\mathbf{k}}) - \mathbf{q} \cdot \nabla_{\mathbf{k}'} \varepsilon_{\mathbf{k}'}|_{\mathbf{k}'=\mathbf{k}+\frac{\mathbf{q}}{2}} \right\} a_{\mathbf{k}+\frac{\mathbf{q}}{2}}^\dagger a_{\mathbf{k}}. \quad (41)$$

The right hand side of Eq. (41) vanishes identically and we obtain the familiar continuity equation

$$\frac{dn_{\mathbf{q}}}{dt} - i\mathbf{q} \cdot \mathbf{J}_{\mathbf{q}} = 0, \quad \text{as } \mathbf{q} \rightarrow 0. \quad (42)$$

### B. $f$ -sum rule

In general, the  $f$ -sum rule can take a complicated form for lattices, especially for momenta  $\mathbf{q}$  near the lattice spacing. However, we are only interested in the long-wavelength limit in this work, where the  $f$ -sum rule becomes simple and familiar. In particular, near the energy band minimum, the dispersion relation typically reduces to a parabolic function,

$$\varepsilon_{\mathbf{k}} = \frac{\hbar^2 \mathbf{k}^2}{2m} + \mathcal{O}(\mathbf{k}^4), \quad (43)$$

where the effective mass  $1/m = \frac{1}{\hbar^2} \frac{\partial^2 \varepsilon_{\mathbf{k}}}{\partial k^2} \big|_{\mathbf{k}=0}$  becomes independent of momentum  $\mathbf{k}$ . Neglecting the higher order corrections in Eq.(43), the current operator in Eq. (38) reduces to

$$\mathbf{J}_{\mathbf{q}} = \frac{1}{\mathcal{V}} \frac{\hbar}{m} \sum_{\mathbf{k}} \left( \mathbf{k} + \frac{\mathbf{q}}{2} \right) a_{\mathbf{k}+\mathbf{q}}^\dagger a_{\mathbf{k}}, \quad (44)$$

which is the familiar continuum form.

Ultimately, the  $f$ -sum rule can reliably computed from the integral of longitudinal current-current response over frequency, which we now show reduces to a simple closed-form expression.

From the continuity equation Eq. (42) we can re-express  $n(\mathbf{q}, t)$

$$n_{\mathbf{q}}(t) - n_{\mathbf{q}}(-\infty) = i\mathbf{q} \cdot \int_{-\infty}^t \mathbf{J}_{\mathbf{q}}(t') dt'. \quad (45)$$

The integral on the right-hand side can be expressed as an equal-time commutator,

$$\begin{aligned} & \int_{-\infty}^{+\infty} \hat{\chi}_{\mathbf{q}}^{LL}(t, t') dt' \\ &= \frac{i\mathcal{V}}{\hbar(\mathbf{q} \cdot \mathbf{q})} \int_{-\infty}^t [\mathbf{q} \cdot \mathbf{J}_{\mathbf{q}}^\dagger(t), \mathbf{q} \cdot \mathbf{J}_{\mathbf{q}}(t')] dt' \\ &= \frac{i\mathcal{V}}{\hbar(\mathbf{q} \cdot \mathbf{q})} \left[ \mathbf{q} \cdot \mathbf{J}_{\mathbf{q}}^\dagger(t), \mathbf{q} \cdot \int_{-\infty}^t \mathbf{J}_{\mathbf{q}}(t') dt' \right] \\ &= \frac{\mathcal{V}}{\hbar(\mathbf{q} \cdot \mathbf{q})} ([\mathbf{q} \cdot \mathbf{J}_{\mathbf{q}}^\dagger(t), n_{\mathbf{q}}(t)] - [\mathbf{q} \cdot \mathbf{J}_{\mathbf{q}}^\dagger(t), n_{\mathbf{q}}(-\infty)]) \\ &= \frac{\mathcal{V}}{\hbar(\mathbf{q} \cdot \mathbf{q})} [\mathbf{q} \cdot \mathbf{J}_{\mathbf{q}}^\dagger(t), n_{\mathbf{q}}(t)] \\ &= \frac{\mathcal{V}}{\hbar(\mathbf{q} \cdot \mathbf{q})} e^{\frac{i\mathbf{q}t}{\hbar}} [\mathbf{q} \cdot \mathbf{J}_{\mathbf{q}}^\dagger, n_{\mathbf{q}}] e^{-\frac{i\mathbf{q}t}{\hbar}}, \end{aligned} \quad (46)$$

where the term  $[\mathbf{q} \cdot \mathbf{J}_{\mathbf{q}}^\dagger(t), n_{\mathbf{q}}(-\infty)]$  is neglected because it represents a correlation across arbitrarily long time, which must decay to zero.

In the continuous limit of Eq.(44), the commutator further reduces

$$\begin{aligned} & [\mathbf{q} \cdot \mathbf{J}_{\mathbf{q}}^\dagger, n_{\mathbf{q}}] \\ &= \frac{1}{\mathcal{V}^2} \frac{\hbar}{m} \sum_{\mathbf{k}\mathbf{k}'} \left( \frac{\mathbf{q} \cdot \mathbf{q}}{2} + \mathbf{k} \cdot \mathbf{q} \right) [a_{\mathbf{k}}^\dagger a_{\mathbf{k}+\mathbf{q}}, a_{\mathbf{k}'+\mathbf{q}}^\dagger a_{\mathbf{k}'}] \\ &= \frac{1}{\mathcal{V}^2} \frac{\hbar}{m} \sum_{\mathbf{k}\mathbf{k}'} \left( \frac{\mathbf{q} \cdot \mathbf{q}}{2} + \mathbf{k} \cdot \mathbf{q} \right) (a_{\mathbf{k}}^\dagger a_{\mathbf{k}'} \delta_{\mathbf{k}\mathbf{k}'} - a_{\mathbf{k}'+\mathbf{q}}^\dagger a_{\mathbf{k}+\mathbf{q}} \delta_{\mathbf{k}\mathbf{k}'} ) \\ &= \frac{1}{\mathcal{V}^2} \frac{\hbar}{m} \sum_{\mathbf{k}} \left( \frac{\mathbf{q} \cdot \mathbf{q}}{2} + \mathbf{k} \cdot \mathbf{q} \right) (n_{\mathbf{k}} - n_{\mathbf{k}+\mathbf{q}}) \\ &= \frac{1}{\mathcal{V}^2} \frac{\hbar(\mathbf{q} \cdot \mathbf{q})}{m} \sum_{\mathbf{k}} \hat{n}_{\mathbf{k}} \\ &= \frac{1}{\mathcal{V}^2} \frac{\hbar N}{m} \mathbf{q} \cdot \mathbf{q}. \end{aligned} \quad (47)$$

Combining Eq. (47) and Eq. (46), we obtain the particularly simple

$$\int_{-\infty}^{+\infty} \hat{\chi}_{\mathbf{q}}^{LL}(t, t') dt' = \frac{N(t)}{m\mathcal{V}}. \quad (48)$$

Notice that the equal-time commutator in Eq.(46) has reduced the total longitudinal response in Eq.(48) to a single local time-dependent function of the total density. Of course, for systems with total particle conservation, such as studied in this work, the right-side of Eq.(48) is time-independent.

#### IV. DRESSED CURRENT AND SUPERFLUID DENSITY

##### A. Definition and form of dressed current

In order to isolate and study different components of the current-current response in the low-frequency limit, we must identify long-lived contributions to the response. The only operators that evolve trivially in time are those that are simultaneously diagonalized with the Hamiltonian.

To that end, we define the current operator  $\tilde{\mathbf{J}}$  for the dressed particles in the Heisenberg picture through the time derivative of the corresponding dressed polarization operator  $\tilde{\Pi}$ ,

$$\tilde{\Pi} = \sum_{\mathbf{R}} \mathbf{R} \tilde{a}_{\mathbf{R}}^{\dagger} \tilde{a}_{\mathbf{R}} \quad (49)$$

$$\Rightarrow \tilde{\mathbf{J}} = \frac{d\tilde{\Pi}}{dt} = \frac{1}{i\hbar} [\tilde{\Pi}, H], \quad (50)$$

Notice that the diagonal representation of Eq.(3) can be additively separated into  $\lambda$ -body parts

$$H = \sum_{\lambda=1}^N H^{(\lambda)} = \sum_{\mathbf{k}_1} \epsilon_{\mathbf{k}_1} \tilde{a}_{\mathbf{k}_1}^{\dagger} \tilde{a}_{\mathbf{k}_1} + \frac{1}{2} \sum_{\mathbf{k}_1 \mathbf{k}_2} \epsilon_{\mathbf{k}_1 \mathbf{k}_2} \tilde{a}_{\mathbf{k}_1}^{\dagger} \tilde{a}_{\mathbf{k}_2}^{\dagger} \tilde{a}_{\mathbf{k}_2} \tilde{a}_{\mathbf{k}_1} + \cdots + \frac{1}{N!} \sum_{\mathbf{k}_1 \cdots \mathbf{k}_N} \epsilon_{\mathbf{k}_1 \cdots \mathbf{k}_N} \tilde{a}_{\mathbf{k}_1}^{\dagger} \cdots \tilde{a}_{\mathbf{k}_N}^{\dagger} \tilde{a}_{\mathbf{k}_N} \cdots \tilde{a}_{\mathbf{k}_1}, \quad (51)$$

and that this separation can be carried over into the definition of the current operator

$$\tilde{\mathbf{J}} = \sum_{\lambda=1}^N \tilde{\mathbf{J}}^{(\lambda)} = \frac{1}{i\hbar} \sum_{\lambda=1}^N [\tilde{\Pi}, H^{(\lambda)}], \quad (52)$$

where we have used the fact that each dressed particle shares its real-space center  $\mathbf{R}$  with the corresponding local bare particle due to the one-to-one mapping between real space operators,

$$\tilde{a}_{\mathbf{R}}^{\dagger} = U^{\dagger} a_{\mathbf{R}}^{\dagger} U, \quad (53)$$

consistent with Eq.(4).

The definition of the dressed current  $\tilde{\mathbf{J}}$  in Eq.(50) properly encodes the hopping of each particle's center as well. For example, the one-body  $\lambda = 1$  part of the dressed current is simply

$$\begin{aligned} \tilde{\mathbf{J}}^{(1)} &= \frac{1}{i\hbar} \left[ \sum_{\mathbf{R}} \mathbf{R} \tilde{a}_{\mathbf{R}}^{\dagger} \tilde{a}_{\mathbf{R}}, \sum_{\mathbf{k}_1} \epsilon_{\mathbf{k}_1} \tilde{a}_{\mathbf{k}_1}^{\dagger} \tilde{a}_{\mathbf{k}_1} \right] \\ &= \frac{1}{i\hbar} \left[ \sum_{\mathbf{R}} \mathbf{R} \tilde{a}_{\mathbf{R}}^{\dagger} \tilde{a}_{\mathbf{R}}, \sum_{\mathbf{R}_1 \mathbf{R}'_1} \tilde{a}_{\mathbf{R}_1}^{\dagger} \left( \sum_{\mathbf{k}_1} \langle \mathbf{R}_1 | \mathbf{k}_1 \rangle \epsilon_{\mathbf{k}_1} \langle \mathbf{k}_1 | \mathbf{R}'_1 \rangle \right) \tilde{a}_{\mathbf{R}'_1} \right] \\ &\equiv \frac{1}{i\hbar} \sum_{\mathbf{R}_1 \mathbf{R}'_1} (\mathbf{R}_1 - \mathbf{R}'_1) \epsilon_{\mathbf{R}_1 \mathbf{R}'_1} \tilde{a}_{\mathbf{R}_1}^{\dagger} \tilde{a}_{\mathbf{R}'_1} \\ &\equiv \sum_{\mathbf{R}_1 \mathbf{R}'_1} \mathbf{J}_{\mathbf{R}_1 \mathbf{R}'_1} \tilde{a}_{\mathbf{R}_1}^{\dagger} \tilde{a}_{\mathbf{R}'_1}, \end{aligned} \quad (54)$$

where  $\mathbf{J}_{\mathbf{R}_1 \mathbf{R}'_1} \tilde{a}_{\mathbf{R}_1}^\dagger \tilde{a}_{\mathbf{R}'_1}$  represents the dressed one-body current from site  $\mathbf{R}'_1$  to site  $\mathbf{R}_1$  located at  $(\mathbf{R}_1 + \mathbf{R}'_1)/2$ . Transforming to momentum space we find the familiar

$$\tilde{\mathbf{J}}_{\mathbf{q}}^{(1)} \equiv \frac{1}{\mathcal{V}} \sum_{\mathbf{R}_1 \mathbf{R}'_1} e^{i\mathbf{q} \cdot (\mathbf{R}_1 + \mathbf{R}'_1)/2} \mathbf{J}_{\mathbf{R}_1 \mathbf{R}'_1} \tilde{a}_{\mathbf{R}_1}^\dagger \tilde{a}_{\mathbf{R}'_1} \quad (55)$$

$$= \frac{1}{\hbar \mathcal{V}} \sum_{\mathbf{k}_1} (\nabla_{\mathbf{p}} \epsilon_{\mathbf{p}}) |_{\mathbf{p}=\mathbf{k}_1+\mathbf{q}/2} \tilde{a}_{\mathbf{k}_1+\mathbf{q}}^\dagger \tilde{a}_{\mathbf{k}_1}. \quad (56)$$

The general  $\lambda$ -body contribution  $\tilde{\mathbf{J}}_{\mathbf{q}}^{(\lambda)}$  is

$$\tilde{\mathbf{J}}_{\mathbf{q}}^{(\lambda)} = \frac{\lambda}{\lambda!} \frac{1}{\hbar \mathcal{V}} \sum_{\mathbf{k}_1 \dots \mathbf{k}_\lambda} \tilde{a}_{\mathbf{k}_1+\mathbf{q}}^\dagger (\nabla_{\mathbf{k}} \epsilon_{\mathbf{k} \mathbf{k}_2 \dots \mathbf{k}_\lambda}) |_{\mathbf{k}=\mathbf{k}_1+\mathbf{q}/2} \tilde{a}_{\mathbf{k}_2}^\dagger \dots \tilde{a}_{\mathbf{k}_\lambda}^\dagger \tilde{a}_{\mathbf{k}_\lambda} \dots \tilde{a}_{\mathbf{k}_2} \tilde{a}_{\mathbf{k}_1}, \quad (57)$$

and therefore the total  $\mathbf{q}$ -component of the dressed current operator is finally

$$\tilde{\mathbf{J}}_{\mathbf{q}} = \frac{1}{\mathcal{V}} \sum_{\mathbf{k}_1} \tilde{a}_{\mathbf{k}_1+\mathbf{q}}^\dagger \tilde{\mathbf{v}}_{\mathbf{k}_1+\frac{\mathbf{q}}{2}} \tilde{a}_{\mathbf{k}_1} \quad (58)$$

$$\tilde{\mathbf{v}}_{\mathbf{k}} \equiv \frac{1}{\hbar} \nabla_{\mathbf{k}} \left( \epsilon_{\mathbf{k}} + \sum_{\mathbf{k}_2} \epsilon_{\mathbf{k} \mathbf{k}_2} \tilde{a}_{\mathbf{k}_2}^\dagger \tilde{a}_{\mathbf{k}_2} + \frac{1}{2!} \sum_{\mathbf{k}_2 \mathbf{k}_3} \epsilon_{\mathbf{k} \mathbf{k}_2 \mathbf{k}_3} \tilde{a}_{\mathbf{k}_2}^\dagger \tilde{a}_{\mathbf{k}_3}^\dagger \tilde{a}_{\mathbf{k}_3} \tilde{a}_{\mathbf{k}_2} + \dots + \frac{1}{(N-1)!} \sum_{\mathbf{k}_2 \dots \mathbf{k}_N} \epsilon_{\mathbf{k} \mathbf{k}_2 \dots \mathbf{k}_N} \tilde{a}_{\mathbf{k}_2}^\dagger \dots \tilde{a}_{\mathbf{k}_N}^\dagger \tilde{a}_{\mathbf{k}_N} \dots \tilde{a}_{\mathbf{k}_2} \right), \quad (59)$$

where  $\tilde{\mathbf{v}}_{\mathbf{k}}$  is the velocity of the dressed particle of corresponding momentum  $\mathbf{k}$ . Note that the gradient in Eq.(59) is taken with respect to the combined kinetic energy and self-energy.

The rotational symmetry of the underlying Hamiltonian ensures that, in the long-wavelength limit  $\mathbf{k} \rightarrow \mathbf{0}$ , the direction of velocity  $\tilde{\mathbf{v}}_{\mathbf{k}}$  is determined by the underlying momentum  $\mathbf{k}$

$$\tilde{\mathbf{v}}_{\mathbf{k}} = \tilde{v}_{\mathbf{k}} \frac{\mathbf{k}}{k}, \quad (60)$$

with corresponding speed  $\tilde{v}_{\mathbf{k}}$ .

Additionally, since the many-body terms are of finite correlation length, the long-wavelength limit  $\mathbf{q} \rightarrow \mathbf{0}$  will filter out such short range correlations leaving only the kinetic part of the dressed current. Recalling that the dressed particles carry the same kinematic velocity as the bare particles in this limit, the dressed current Eq.(58) must reduce to

$$\tilde{\mathbf{J}}_{\mathbf{q}} \xrightarrow{\mathbf{q} \rightarrow \mathbf{0}} \frac{1}{\mathcal{V}} \sum_{\mathbf{k}} \frac{\hbar \mathbf{k}}{m} \tilde{a}_{\mathbf{k}}^\dagger \tilde{a}_{\mathbf{k}}. \quad (61)$$

In essence, the self-energy terms in Eq.(59) originate from the many-body part of  $H_{\text{diag}}$ , and therefore only account for the velocity modulation at short wavelength due to short-range quantum fluctuation. As the superfluid response is a long-wavelength phenomenon, we neglect such short range effects.

## B. continuity equation for dressed current

We now show that the dressed current as defined above obeys the familiar equation of continuity in the long-wavelength limit. Similar to the dressed current operator of Eq.(52) in the previous section, by using Eq.(51) we can separate the Heisenberg equation of motion for the density operator into  $\lambda$ -body parts

$$\frac{d\tilde{n}_{\mathbf{R}}}{dt} = \frac{1}{i\hbar} [\tilde{n}_{\mathbf{R}}, H_{\text{diag}}] = \frac{1}{i\hbar} \sum_{\lambda=1}^N [\tilde{n}_{\mathbf{R}}, H^{(\lambda)}], \quad (62)$$

due to the associativity of the commutator. We can therefore examine an arbitrary  $\lambda$ -body term to determine the form of the continuity equation. For example, from Eq.(62)

$$\begin{aligned} \frac{d\tilde{n}_{\mathbf{R}}^{(\lambda)}}{dt} &= \frac{1}{i\hbar} [\tilde{n}_{\mathbf{R}}, H^{(\lambda)}] \\ &= \frac{1}{i\hbar \lambda!} \left[ \tilde{a}_{\mathbf{R}}^\dagger \tilde{a}_{\mathbf{R}}, \sum_{\mathbf{k}_1, \dots, \mathbf{k}_\lambda} \epsilon_{\mathbf{k}_1, \dots, \mathbf{k}_\lambda} \tilde{a}_{\mathbf{k}_1}^\dagger \dots \tilde{a}_{\mathbf{k}_\lambda}^\dagger \tilde{a}_{\mathbf{k}_\lambda} \dots \tilde{a}_{\mathbf{k}_1} \right] \\ &= \frac{1}{i\hbar} \sum_{\mathbf{R}'} \left( \tilde{a}_{\mathbf{R}}^\dagger F^{(\lambda)}(\mathbf{R} \mathbf{R}') \tilde{a}_{\mathbf{R}'} - \tilde{a}_{\mathbf{R}'}^\dagger F^{(\lambda)}(\mathbf{R}' \mathbf{R}) \tilde{a}_{\mathbf{R}} \right) \end{aligned} \quad (63)$$

where  $F^{(1)}(\mathbf{R}\mathbf{R}') = \sum_{\mathbf{k}_1} \langle \mathbf{R} | \mathbf{k}_1 \rangle \varepsilon_{\mathbf{k}_1} \langle \mathbf{k}_1 | \mathbf{R}' \rangle$ ,  $F^{(\lambda>1)}(\mathbf{R}\mathbf{R}') = \frac{1}{(\lambda-1)!} \sum_{\mathbf{k}_2 \dots \mathbf{k}_\lambda} \langle \mathbf{R} | \mathbf{k}_2 \dots \mathbf{k}_\lambda | \hat{h}^{(\lambda)} | \mathbf{R}', \mathbf{k}_2 \dots \mathbf{k}_\lambda \rangle \tilde{a}_{\mathbf{k}_2}^\dagger \dots \tilde{a}_{\mathbf{k}_\lambda}^\dagger \tilde{a}_{\mathbf{k}_\lambda} \dots \tilde{a}_{\mathbf{k}_2}$ , and  $\hat{h}^{(\lambda>1)} \equiv \sum_{\mathbf{k}_2 \dots \mathbf{k}_\lambda} |\mathbf{k}_2 \dots \mathbf{k}_\lambda \rangle \varepsilon_{\mathbf{k}_2 \dots \mathbf{k}_\lambda} \langle \mathbf{k}_\lambda \dots \mathbf{k}_2 |$ .

Similarly, from Eq.(52) the current operator becomes

$$\tilde{\mathbf{J}} = \sum_{\lambda=1}^N \frac{1}{i\hbar} \sum_{\mathbf{R}\mathbf{R}'} \tilde{a}_{\mathbf{R}}^\dagger F^{(\lambda)}(\mathbf{R}\mathbf{R}') \tilde{a}_{\mathbf{R}'}. \quad (64)$$

Combining symmetric terms in the dressed current,

$$\tilde{\mathbf{J}}_{\mathbf{R}\mathbf{R}'} + \tilde{\mathbf{J}}_{\mathbf{R}'\mathbf{R}} = \frac{1}{i\hbar} \sum_{\lambda=1}^N \delta_{\mathbf{R}\mathbf{R}'} \left( \tilde{a}_{\mathbf{R}}^\dagger F^{(\lambda)}(\mathbf{R}\mathbf{R}') \tilde{a}_{\mathbf{R}'} - \tilde{a}_{\mathbf{R}'}^\dagger F^{(\lambda)}(\mathbf{R}'\mathbf{R}) \tilde{a}_{\mathbf{R}} \right), \quad (65)$$

we can directly compare terms in Eq. (63) with Eq. (65) to find the simple form

$$\frac{d\tilde{n}_{\mathbf{R}}}{dt} + \sum_{\mathbf{R}'} \frac{\delta_{\mathbf{R}'\mathbf{R}}}{|\delta_{\mathbf{R}'\mathbf{R}}|^2} \cdot (\tilde{\mathbf{J}}_{\mathbf{R}\mathbf{R}'} + \tilde{\mathbf{J}}_{\mathbf{R}'\mathbf{R}}) = 0. \quad (66)$$

Eq.(66) is the continuity equation for dressed current, and in the long-wavelength limit,  $\mathbf{q} \rightarrow 0$ , it reduces to the familiar form

$$\frac{d\tilde{n}_{\mathbf{q}}}{dt} - i\mathbf{q} \cdot \tilde{\mathbf{J}}_{\mathbf{q}} = 0. \quad (67)$$

Below, the continuity equation for the dressed particles in Eq.(67) in the long-wavelength limit will be confirmed by the rigorous enforcement of the  $f$ -sum rule in the dynamic current-current response.

### C. Superfluid component of response function

Above we identified that the dressed current defined in Eq.(50) satisfies the familiar continuity equation in the long-wavelength limit via Eq.(67). Therefore, it is safe to replace the  $\mathbf{q}$ -component of the standard current in Eq.(38) with that of the corresponding dressed current in Eq.(58) in the Kubo formula for current-current response.

Recall the dressed current from Eq.(58)

$$\tilde{\mathbf{J}}_{\mathbf{q}}(t) = \frac{1}{\mathcal{V}} \sum_{\mathbf{k}} \frac{(\mathbf{k} + \frac{\mathbf{q}}{2})}{|\mathbf{k} + \frac{\mathbf{q}}{2}|} \tilde{a}_{\mathbf{k}+\mathbf{q}}^\dagger(t) \tilde{v}_{\mathbf{k}+\frac{\mathbf{q}}{2}}(t) \tilde{a}_{\mathbf{k}}(t). \quad (68)$$

It is convenient to separate the current into longitudinal  $\tilde{\mathbf{J}}_{\mathbf{q}}^L = \frac{1}{q^2} \mathbf{q}(\mathbf{q} \cdot \tilde{\mathbf{J}}_{\mathbf{q}})$  and transverse  $\tilde{\mathbf{J}}_{\mathbf{q}}^T = -\frac{1}{q^2} \mathbf{q} \times (\mathbf{q} \times \tilde{\mathbf{J}}_{\mathbf{q}})$  components

$$\tilde{\mathbf{J}}_{\mathbf{q}}^L(t) = \frac{1}{\mathcal{V}} \sum_{\mathbf{k}} \frac{1}{|\mathbf{k} + \frac{\mathbf{q}}{2}|} \left( \frac{\mathbf{q}}{2} + \frac{\mathbf{q}(\mathbf{q} \cdot \mathbf{k})}{q^2} \right) \tilde{a}_{\mathbf{k}+\mathbf{q}}^\dagger(t) \tilde{v}_{\mathbf{k}+\frac{\mathbf{q}}{2}}(t) \tilde{a}_{\mathbf{k}}(t) \quad (69)$$

$$\begin{aligned} \tilde{\mathbf{J}}_{\mathbf{q}}^T(t) &= \frac{1}{\mathcal{V}} \sum_{\mathbf{k}} \frac{1}{|\mathbf{k} + \frac{\mathbf{q}}{2}|} \hat{\alpha} \cdot \left( \mathbf{k} - \frac{\mathbf{q}(\mathbf{q} \cdot \mathbf{k})}{q^2} \right) \tilde{a}_{\mathbf{k}+\mathbf{q}}^\dagger(t) \tilde{v}_{\mathbf{k}+\frac{\mathbf{q}}{2}}(t) \tilde{a}_{\mathbf{k}}(t) \\ &= \frac{1}{\mathcal{V}} \sum_{\mathbf{k}} \frac{1}{|\mathbf{k} + \frac{\mathbf{q}}{2}|} (\hat{\alpha} \cdot \mathbf{k}) \tilde{a}_{\mathbf{k}+\mathbf{q}}^\dagger(t) \tilde{v}_{\mathbf{k}+\frac{\mathbf{q}}{2}}(t) \tilde{a}_{\mathbf{k}}(t) \end{aligned} \quad (70)$$

Here,  $\hat{\alpha}$  is the unit vector along a transverse direction, with the relation  $\hat{\alpha} \cdot \mathbf{q} = 0$ . From the standard Kubo formula, the response function of the susceptibility can be written via projections of the momentum- $\mathbf{q}$  component of the current operator  $\tilde{\mathbf{J}}_{\mathbf{q}}(t)$  along the  $\alpha$  and  $\beta$  directions

$$\tilde{\chi}^{\alpha\beta}(\mathbf{r}\mathbf{t}; \mathbf{r}'\mathbf{t}') = \frac{i}{\hbar} \theta(t-t') \left[ \tilde{J}^{\alpha}(\mathbf{r}, t), \tilde{J}^{\beta}(\mathbf{r}', t') \right] \quad (71)$$

$$\begin{aligned} \tilde{\chi}_{\mathbf{q}}^{\alpha\beta}(t, t') &= \frac{1}{\mathcal{V}} \int \tilde{\chi}^{\alpha\beta}(\mathbf{r}\mathbf{t}; \mathbf{r}'\mathbf{t}') e^{i\mathbf{q} \cdot (\mathbf{r} - \mathbf{r}')} d^3(\mathbf{r} - \mathbf{r}') \\ &= \frac{i\mathcal{V}}{\hbar} \theta(t-t') \left[ \tilde{J}_{\mathbf{q}}^{\alpha\dagger}(t), \tilde{J}_{\mathbf{q}}^{\beta}(t') \right] \end{aligned} \quad (72)$$

$$\begin{aligned} \tilde{\chi}_{\mathbf{q}}^{\alpha\beta}(t, \omega = 0) &= \int \tilde{\chi}_{\mathbf{q}}^{\alpha\beta}(t, t') dt' \\ &= \frac{i\mathcal{V}}{\hbar} \int \theta(t-t') \left[ \tilde{J}_{\mathbf{q}}^{\alpha\dagger}(t), \tilde{J}_{\mathbf{q}}^{\beta}(t') \right] dt' \end{aligned} \quad (73)$$

Correspondingly, the longitudinal response becomes

$$\begin{aligned}
\tilde{\chi}_{\mathbf{q}}^{LL}(t, t') &= \frac{i\mathcal{V}}{\hbar} \theta(t-t') [\tilde{J}_{\mathbf{q}}^{L\dagger}(t), \tilde{J}_{\mathbf{q}}^L(t')] \\
&= \frac{i\mathcal{V}}{\hbar} \theta(t-t') \sum_{\mathbf{k}, \mathbf{k}'} \frac{1}{|\mathbf{k} + \frac{\mathbf{q}}{2}|^2} \left( \frac{q^2}{4} + \frac{\mathbf{q} \cdot (\mathbf{k} + \mathbf{k}')}{2} + \frac{(\mathbf{q} \cdot \mathbf{k})(\mathbf{q} \cdot \mathbf{k}')}{q^2} \right) [\tilde{a}_{\mathbf{k}}^\dagger(t) \tilde{v}_{\mathbf{k} + \frac{\mathbf{q}}{2}}^\dagger(t) \tilde{a}_{\mathbf{k} + \mathbf{q}}(t), \tilde{a}_{\mathbf{k}' + \mathbf{q}}^\dagger(t') \tilde{v}_{\mathbf{k}' + \frac{\mathbf{q}}{2}}^\dagger(t') \tilde{a}_{\mathbf{k}'}(t')] \\
&= \frac{i\mathcal{V}}{\hbar} \theta(t-t') \sum_{\mathbf{k}} \frac{1}{|\mathbf{k} + \frac{\mathbf{q}}{2}|^2} \left( \frac{q^2}{4} + \mathbf{q} \cdot \mathbf{k} + \left( \frac{\mathbf{q}}{q} \cdot \mathbf{k} \right)^2 \right) [\tilde{a}_{\mathbf{k}}^\dagger(t) \tilde{v}_{\mathbf{k} + \frac{\mathbf{q}}{2}}^\dagger(t) \tilde{a}_{\mathbf{k} + \mathbf{q}}(t), \tilde{a}_{\mathbf{k} + \mathbf{q}}^\dagger(t') \tilde{v}_{\mathbf{k} + \frac{\mathbf{q}}{2}}^\dagger(t') \tilde{a}_{\mathbf{k}}(t')], \tag{74}
\end{aligned}$$

and the transverse response becomes

$$\begin{aligned}
\tilde{\chi}_{\mathbf{q}}^{TT}(t, t') &= \frac{i\mathcal{V}}{\hbar} \theta(t-t') [\tilde{J}_{\mathbf{q}}^{T\alpha\dagger}(t), \tilde{J}_{\mathbf{q}}^{T\alpha}(t')] \\
&= \frac{i\mathcal{V}}{\hbar} \theta(t-t') \sum_{\mathbf{k}, \mathbf{k}'} \frac{1}{|\mathbf{k} + \frac{\mathbf{q}}{2}|^2} (\hat{\alpha} \cdot \mathbf{k})(\hat{\alpha} \cdot \mathbf{k}') [\tilde{a}_{\mathbf{k}}^\dagger(t) \tilde{v}_{\mathbf{k} + \frac{\mathbf{q}}{2}}^\dagger(t) \tilde{a}_{\mathbf{k} + \mathbf{q}}(t), \tilde{a}_{\mathbf{k}' + \mathbf{q}}^\dagger(t') \tilde{v}_{\mathbf{k}' + \frac{\mathbf{q}}{2}}^\dagger(t') \tilde{a}_{\mathbf{k}'}(t')] \\
&= \frac{i\mathcal{V}}{\hbar} \theta(t-t') \sum_{\mathbf{k}} \frac{1}{|\mathbf{k} + \frac{\mathbf{q}}{2}|^2} (\hat{\alpha} \cdot \mathbf{k})^2 [\tilde{a}_{\mathbf{k}}^\dagger(t) \tilde{v}_{\mathbf{k} + \frac{\mathbf{q}}{2}}^\dagger(t) \tilde{a}_{\mathbf{k} + \mathbf{q}}(t), \tilde{a}_{\mathbf{k} + \mathbf{q}}^\dagger(t') \tilde{v}_{\mathbf{k} + \frac{\mathbf{q}}{2}}^\dagger(t') \tilde{a}_{\mathbf{k}}(t')]. \tag{75}
\end{aligned}$$

Recall that the time evolution of an eigenoperator of the Hamiltonian, such as  $\tilde{a}_{\mathbf{k}}^\dagger(t)$ , is a trivial overall phase factor. In addition, terms with  $\mathbf{k} = \mathbf{0}$  or  $\mathbf{k} = -\mathbf{q}$  directly involve zero momentum, and only contribute to the longitudinal response. For the remaining terms, in the long-wavelength limit  $\mathbf{q} \rightarrow 0$ , the longitudinal response becomes

$$\lim_{\mathbf{q} \rightarrow 0} \tilde{\chi}_{\mathbf{q}}^{LL}(t, t') = \frac{i\mathcal{V}}{\hbar} \theta(t-t') \sum_{\mathbf{k} \neq \mathbf{0}, -\mathbf{q}} \frac{1}{|\mathbf{k} + \frac{\mathbf{q}}{2}|^2} \left( \frac{\mathbf{q}}{q} \cdot \mathbf{k} \right)^2 [\tilde{a}_{\mathbf{k}}^\dagger(t) \tilde{v}_{\mathbf{k} + \frac{\mathbf{q}}{2}}^\dagger(t) \tilde{a}_{\mathbf{k} + \mathbf{q}}(t), \tilde{a}_{\mathbf{k} + \mathbf{q}}^\dagger(t') \tilde{v}_{\mathbf{k} + \frac{\mathbf{q}}{2}}^\dagger(t') \tilde{a}_{\mathbf{k}}(t')], \tag{76}$$

where  $\hat{\mathbf{q}} = \frac{\mathbf{q}}{q}$  is the unit vector along the  $\mathbf{q}$ -direction. As  $\mathbf{q} \rightarrow \mathbf{0}$ , the longitudinal response terms in Eq.(76) are equal to those of the transverse response in Eq.(75) due to the rotational symmetry of the system.

On the other hand, similar to the bare current<sup>4</sup>, a standard vector analysis of the susceptibility indicates that in Eq.(68) the contribution directly involving zero momentum,

$$\tilde{\mathbf{J}}_{\mathbf{q}}^s = \frac{1}{\mathcal{V}} \frac{\mathbf{q}}{q} (\tilde{a}_{\mathbf{q}}^\dagger \tilde{v}_{\frac{\mathbf{q}}{2}} \tilde{a}_{\mathbf{0}} - \tilde{a}_{\mathbf{0}}^\dagger \tilde{v}_{-\frac{\mathbf{q}}{2}} \tilde{a}_{-\mathbf{q}}), \tag{77}$$

is the only part that produces the longitudinal-only response missing in the transverse response. In summary, the superfluid response is rigorously tied to the excitation involving dressed particles of zero momentum. Again, while the identification of the longitudinal-only component is similar to the standard description using the bare particles, it is the long-lived nature of the dressed particles that validates  $\tilde{\mathbf{J}}_{\mathbf{q}}^s$  for describing superfluidity.

$$\begin{aligned}
\frac{\rho_s}{m^2} &= \lim_{\mathbf{q} \rightarrow 0} \tilde{\chi}_{\mathbf{q}}^s(t, \omega = 0) \\
&= \lim_{\mathbf{q} \rightarrow 0} (\chi_{\mathbf{q}}^{LL}(t, \omega = 0) - \chi_{\mathbf{q}}^{TT}(t, \omega = 0)) \\
&= \lim_{\mathbf{q} \rightarrow 0} \frac{i\mathcal{V}}{\hbar} \int \theta(t-t') [\tilde{\mathbf{J}}_{\mathbf{q}}^{s\dagger}(t), \tilde{\mathbf{J}}_{\mathbf{q}}^s(t')] dt' \tag{78}
\end{aligned}$$

$$= \lim_{\mathbf{q} \rightarrow 0} \frac{\mathcal{V}}{\hbar q^2} [\mathbf{q} \cdot \tilde{\mathbf{J}}_{\mathbf{q}}^{s\dagger}(t), \tilde{n}_{\mathbf{q}}^s(t)] \tag{79}$$

$$\begin{aligned}
&= \lim_{\mathbf{q} \rightarrow 0} \frac{q}{\hbar \mathcal{V} q^2} \left\{ \tilde{a}_{\mathbf{0}}^\dagger(t) \tilde{v}_{\frac{\mathbf{q}}{2}}^\dagger(t) \tilde{a}_{\mathbf{0}}(t) - \tilde{a}_{\mathbf{q}}^\dagger(t) \tilde{v}_{\frac{\mathbf{q}}{2}}^\dagger(t) \tilde{a}_{\mathbf{q}}(t) + \tilde{a}_{\mathbf{0}}^\dagger(t) [\tilde{v}_{\frac{\mathbf{q}}{2}}^\dagger(t), \tilde{a}_{\mathbf{q}}^\dagger(t) \tilde{a}_{\mathbf{0}}(t) + \tilde{a}_{\mathbf{0}}^\dagger(t) \tilde{a}_{-\mathbf{q}}(t)] \tilde{a}_{\mathbf{q}}(t) \right. \\
&\quad \left. + \tilde{a}_{\mathbf{0}}^\dagger(t) \tilde{v}_{-\frac{\mathbf{q}}{2}}^\dagger(t) \tilde{a}_{\mathbf{0}}(t) - \tilde{a}_{-\mathbf{q}}^\dagger(t) \tilde{v}_{-\frac{\mathbf{q}}{2}}^\dagger(t) \tilde{a}_{-\mathbf{q}}(t) - \tilde{a}_{-\mathbf{q}}^\dagger(t) [\tilde{v}_{-\frac{\mathbf{q}}{2}}^\dagger(t), \tilde{a}_{\mathbf{q}}^\dagger(t) \tilde{a}_{\mathbf{0}}(t) + \tilde{a}_{\mathbf{0}}^\dagger(t) \tilde{a}_{-\mathbf{q}}(t)] \tilde{a}_{\mathbf{0}}(t) \right\} \\
&= \lim_{\mathbf{q} \rightarrow 0} \frac{1}{\hbar \mathcal{V} q} \left\{ \tilde{a}_{\mathbf{0}}^\dagger(t) [\tilde{v}_{\frac{\mathbf{q}}{2}}^\dagger(t) + \tilde{v}_{-\frac{\mathbf{q}}{2}}^\dagger(t)] \tilde{a}_{\mathbf{0}}(t) - [\tilde{a}_{\mathbf{q}}^\dagger(t) \tilde{v}_{\frac{\mathbf{q}}{2}}^\dagger(t) \tilde{a}_{\mathbf{q}}(t) + \tilde{a}_{-\mathbf{q}}^\dagger(t) \tilde{v}_{-\frac{\mathbf{q}}{2}}^\dagger(t) \tilde{a}_{-\mathbf{q}}(t)] \right\} \tag{80}
\end{aligned}$$

$$+ \tilde{\gamma}_{\frac{\mathbf{q}}{2}}^\dagger(t) \tilde{a}_{\mathbf{q}}^\dagger(t) \tilde{a}_{\mathbf{0}}^\dagger(t) \tilde{a}_{\mathbf{0}}(t) \tilde{a}_{\mathbf{q}}(t) - \tilde{\gamma}_{-\frac{\mathbf{q}}{2}}^\dagger(t) \tilde{a}_{-\mathbf{q}}^\dagger(t) \tilde{a}_{\mathbf{0}}^\dagger(t) \tilde{a}_{\mathbf{0}}(t) \tilde{a}_{-\mathbf{q}}(t) \left\} \tag{81}$$

$$= \lim_{\mathbf{q} \rightarrow 0} \frac{1}{\hbar \mathcal{V} q} \left\{ \tilde{a}_{\mathbf{0}}^\dagger(t) [\tilde{v}_{\frac{\mathbf{q}}{2}}^\dagger(t) + \tilde{v}_{-\frac{\mathbf{q}}{2}}^\dagger(t)] \tilde{a}_{\mathbf{0}}(t) + \mathcal{O}(1) \right\} \tag{82}$$

$$= \frac{1}{\hbar \mathcal{V} q} \left\{ \tilde{a}_{\mathbf{0}}^\dagger(t) \left[ \hbar \left| \frac{\mathbf{q}}{2m} \right| + \hbar - \frac{\mathbf{q}}{2m} \right] \tilde{a}_{\mathbf{0}}(t) + \mathcal{O}(1) \right\} \tag{83}$$

$$= \frac{1}{m \mathcal{V}} [\tilde{a}_{\mathbf{0}}^\dagger(t) \tilde{a}_{\mathbf{0}}(t) + \mathcal{O}(1)],$$

Where  $\tilde{\gamma}_{\mathbf{k}} \equiv \nabla_{\mathbf{k}} \cdot \tilde{\mathbf{v}}_{\mathbf{k}}$  in Eq.(81). Here the continuity equation of dressed particle Eq.(67) is employed in replacing the integration of  $\mathbf{q} \cdot \tilde{\mathbf{J}}_{\mathbf{q}}^s(t')$  over  $t'$  by  $\tilde{n}_{\mathbf{q}}^s(t)$  in the Eq.(78) to Eq.(79). As indicated in going from Eq.(80) and Eq.(81) to Eq.(82), the occupation number at finite momentum ( $\tilde{a}_{\mathbf{k}}^\dagger \tilde{a}_{\mathbf{k}} \forall \mathbf{k} \neq \mathbf{0}$ ) is of order  $\mathcal{O}(1)$ , which is negligible compared to the condensation number  $\tilde{a}_{\mathbf{0}}^\dagger \tilde{a}_{\mathbf{0}}$  of order  $\mathcal{O}(N)$ . Finally, the long-wavelength limit of the dressed current [i.e. going from Eq.(58 to Eq.(61)] was used to simplify Eq.(82) into Eq.(83).

We thus reach a *rigorous* quantum mechanical identification of the superfluid fraction, in direct one-to-one mapping to the true condensation density fraction,

$$\rho_s/\rho = \tilde{a}_{\mathbf{0}}^\dagger \tilde{a}_{\mathbf{0}}/N \equiv \tilde{N}_0/N. \tag{84}$$

$$\rho_n/\rho = \sum_{\mathbf{k} \neq \mathbf{0}} \tilde{a}_{\mathbf{k}}^\dagger \tilde{a}_{\mathbf{k}}/N. \tag{85}$$

## V. THERMAL FLUCTUATION OF SUPERFLUID DENSITY

### A. Estimate in the grand canonical ensemble

Having identified the superfluid density fraction as directly proportional to the true condensate density  $\rho_s/\rho = \tilde{a}_{\mathbf{0}}^\dagger \tilde{a}_{\mathbf{0}}/N$  in Eq.(84), it is straightforward to estimate the temperature dependence of the true condensate density via the grand canonical ensemble (GCE) using the linear dispersion  $\epsilon_{\mathbf{k}}$  of the particle-hole excitations developed in section IV.

The condensate cannot be studied directly in the GCE, where there is no particle conservation, so the total excited particle statistics are computed instead and an *ad hoc* assumption is made to subtract the result from an assumed well-defined average particle number  $N$

$$\tilde{N}_0 = N - \int d^3\mathbf{k} n_B[\beta(\epsilon_{\mathbf{k}} - \epsilon_0)], \tag{86}$$

where  $\beta = 1/k_B T$  and the chemical potential is pinned to  $\epsilon_0$  in the presence of a condensate.

It is a standard exercise to compute the temperature dependence of the condensate in a 3D system of bosons with a linear

dispersion  $\epsilon_{\mathbf{k}} - \epsilon_0 = v|\mathbf{k}|$ , which gives

$$\tilde{N}_0/N = 1 - \frac{4\pi}{N(v\beta)^3} \int_0^\infty dx x^2 n_B(x) \quad (87)$$

$$= 1 - \frac{8\pi\zeta(3)k_B^3}{Nv^3} T^3, \quad (88)$$

where  $x = \beta v|\mathbf{k}|$  and  $\zeta(3) \approx 1.202$ . Eq.(88) identifies the depletion of the true condensate to be  $\propto T^3$  for the low energy theory developed above. Therefore, by Eq.(84) the depletion of the superfluid density is also  $\propto T^3$  at low temperature.

## B. Derivation in the canonical ensemble

Having solved the particle conserved quantum problem at low energy, we can introduce the effects of finite temperature via an appropriately particle-conserving statistical ensemble such as the canonical ensemble (CE). The CE incorporates the highly relevant scale of total particle number  $N$  at low energy that is fundamentally absent in the GCE, so it should not be too surprising that our formulation of superfluidity at low energy avoids many of the problems plaguing the traditional methods. In fact, it is well-known<sup>5</sup> that the CE and the GCE can produce different macroscopic properties in the presence of a condensate.

Since our system is solved strictly in the  $N$ -particle sector, every many-body state satisfies the one-body constraint

$$N = \tilde{N}_0 + \tilde{N}_e \quad (89)$$

$$\tilde{N}_e = \sum_{\mathbf{p} \neq 0} \tilde{a}_{\mathbf{p}}^\dagger \tilde{a}_{\mathbf{p}}, \quad (90)$$

where  $\tilde{N}_e$  is the sum over excitations above the condensate. Therefore, once the condensate and the excitations are taken together, computing thermal statistics under the constraint in Eq.(89) requires the canonical ensemble.

As shown by Fujiwara et al<sup>6</sup>, the complications of the restricted sum in the partition function of the canonical ensemble

$$Z = \sum_{n_s} \prod_s e^{-\beta \epsilon_s n_s}, \quad (91)$$

can be overcome by introducing a constraint parameter  $t$  to the partition function

$$Z = \frac{1}{2\pi i} \int dt e^{-Nt} \sum_s \left( \sum_{n_s} e^{n_s(t - \beta \epsilon_s)} \right). \quad (92)$$

Choosing the sum over occupation statistics  $n_s$  to run from 0 to  $N$  results in a closed form for the partition function

$$Z = \frac{1}{2\pi i} \int dt \prod_s \left( \frac{1 - e^{-Dz_s}}{1 - e^{-z_s}} \right) \quad (93)$$

$$D = N + 1 \quad (94)$$

$$z_s = \beta \epsilon_s - t, \quad (95)$$

that is extremely well-behaved and smooth. So much so that steepest descent methods can be reliably used to find unique saddle-point values for  $t$  in the large system limit, in great contrast to grand canonical ensemble formulations for bosons.

The saddle-point equation resulting from the above treatment

$$N = \sum_s n_B(z_s) - D n_B(Dz_s) \equiv \sum_s n_G(z_s, N), \quad (96)$$

simply applies the constraint of total particle number  $N$  on the occupation statistics resulting in the ‘Gentile-ter Haar-Wergeland’ distribution function  $n_G$ , which is itself a simple function of the Bose-Einstein distribution function  $n_B$ . Although Eq.(96) may appear superficially similar to the equation in the grand canonical ensemble used to identify the chemical potential, here the occupation of the lowest energy state is explicitly included even in the presence of Bose-Einstein condensation (BEC).

Before studying the statistics required for our fluid responses, it is necessary to recall<sup>6</sup> the relevant saddle-point behavior of  $t$ . For temperatures much larger than the condensation temperature, the saddle-point is below the lowest energy state  $t < \beta \epsilon_0$ . It reaches the lowest energy  $t = \beta \epsilon_0$  precisely when the condensate at  $\epsilon_0$  contains half of the total  $N$  particles  $N_0 = n_G(-t, N) = N/2$ . As the temperature is lowered further, the saddle-point increases, but it is bounded from above  $\beta \epsilon_0 < t < \beta \epsilon_1$ , where  $\epsilon_1$  is the lowest excitation energy. However, as studied previously<sup>6</sup>, the saddle-point  $t$  only approaches its limiting value for extremely

low temperatures, namely when the temperature scale is of the same order as the energy level spacing between  $\varepsilon_0$  and  $\varepsilon_1$ . Our system has a gapless single-particle spectrum given by Eq.(26), so we are interested in temperatures where the condensate is large ( $t > 0$ ) but the temperature scale is much larger than the spacing between low-lying energy levels ( $\beta \ll \varepsilon_1 - \varepsilon_0$ ). In this regime  $\beta \varepsilon_0 < t \ll \beta \varepsilon_1$  the saddle-point at any fixed temperature  $T$  is small  $t \ll 1$ .

In our system the dispersion  $\Omega_k \equiv v|\mathbf{k}|$ , so the lowest energy state is zero ( $\varepsilon_0 = 0$ ), and below we use the notation for the true condensate defined in section IIIA. Simplifying the occupation function  $n_G(z_s)$  for small positive  $t$

$$\tilde{N}_0 = n_G(-t) \approx N - n_B(t) \approx N - \frac{1}{t} \quad (97)$$

$$n_G(\beta \Omega_k - t) \approx n_B(-\beta \Omega_k + t), \quad (98)$$

we use the saddle-point constraint in Eq.(96) and find

$$t \approx \left( \frac{8\pi\zeta(3)}{v^3\beta^3} \right)^{-1}. \quad (99)$$

Returning to the sum rule as discussed in section IIIE, Eq.(84) shows that the true condensate density  $\tilde{N}_0$  is directly proportional to the superfluid density. In our canonical ensemble formulation, the condensate temperature dependence is simply

$$\frac{\rho_s(T)}{\rho} = \frac{\tilde{N}_0(T)}{N} = 1 - AT^3 + \mathcal{O}(T^4) \quad (100)$$

$$A = \frac{8\pi\zeta(3)k_B^3}{Nv^3}. \quad (101)$$

Applying the results in Eqs.(97-99) to the excitations, the leading order normal fluid contribution becomes

$$\frac{\rho_n}{\rho}(T) \approx \int d^3p \, n_G(\omega_p) \approx AT^3 + \mathcal{O}(T^4), \quad (102)$$

where  $A$  is *identical* to that defined in the superfluid depletion of Eq. (101). Therefore, Eqs.(100,102) are consistent with the sum rule yet again

$$\frac{\rho_s}{\rho} + \frac{\rho_n}{\rho} = [1 - AT^3 - \mathcal{O}(T^4)] + [AT^3 + \mathcal{O}(T^4)], \quad (103)$$

which is not surprising given the strict confinement to the  $N$ -particle sector. The above thermal formulation has shown that the thermal depletion of the superfluid density is consistent with the  $f$ -sum rule at finite temperature.

## VI. NO-GO THEOREM FORBIDDING PHONONS FROM REPRESENTING THE NORMAL FLUID

On one hand, the phenomenon of superfluidity generally occurs as dissipationless flow in the presence of dissipative flow, and the latter is required to come to rest (*locally* in position space) with a boundary, in order to establish equilibrium. On the other hand, traditional superfluid theory constructions assume that the non-superfluid part of the system is a so-called ‘gas of phonons,’ in other words an ensemble of waves each of well-defined wavenumber  $\mathbf{k}$ . Such waves could only satisfy a local boundary condition via construction of appropriately localized ‘wave packets’ requiring the superposition of many such waves. As we prove below, this necessary construction is impossible.

In this section, we prove two theorems and then use them to prove a corollary establishing a no-go theorem that renders *any* ensemble formed from “quanta of longitudinal waves”<sup>7</sup> incapable of satisfying the boundary conditions required to describe normal fluid flow as described above. Note that *all* of the assumptions utilized in this section come from prominent established literature<sup>1,8</sup>.

**Theorem 1** *A generic state  $\psi(\mathbf{r})$ , composed of a sum over quanta of longitudinal waves that satisfy a system exhibiting translational symmetry, always satisfies the condition of potential flow  $\nabla \times \mathbf{v} = 0$ .*

**Theorem 2** *The only such state that satisfies both  $\nabla \times \mathbf{v} = 0$  and the boundary condition for a viscous liquid<sup>1</sup>  $\mathbf{v}_{\text{bdry}} = \mathbf{v}_{\text{wall}}$  is a single trivial plane wave  $\psi(\mathbf{r}) = e^{-i\mathbf{k} \cdot \mathbf{r}}$ .*

**Corollary 1** *The (excitation) waves used to generate the state in Theorem 1 do not satisfy Theorem 2 in an arbitrary inertial frame.*

To prove Theorem 1, we first define a generic state composed of a sum over quanta of longitudinal waves<sup>8</sup>

$$\psi(\mathbf{r}) \equiv \sum_{\mathbf{k}} \left( \alpha_{\mathbf{k}} e^{i\mathbf{k} \cdot \mathbf{r}} + \beta_{\mathbf{k}} e^{-i\mathbf{k} \cdot \mathbf{r}} \right), \quad (104)$$

where real inversion-symmetric coefficients  $\alpha_{-\mathbf{k}} = \alpha_{\mathbf{k}}$  and  $\beta_{-\mathbf{k}} = \beta_{\mathbf{k}}$  can be chosen for a translationally invariant liquid with linear or quadratic dispersion at low energy. This state includes those generated via excitations out of a mean-field condensate, for example.

Our goal is to compute the flow  $\mathbf{v}$  of this quantum state

$$\mathbf{v} \equiv \frac{\hbar}{2mi} \left( \psi^* \nabla \psi - \psi \nabla \psi^* \right), \quad (105)$$

where  $m$  is the so-called inertial mass of the state  $\psi$ , followed by the curl of Eq.(105). To this end, it is straightforward to first identify the general conditions on the state itself after applying both

$$\nabla \times \mathbf{v} = \frac{\hbar}{2mi} \nabla \times \left( \psi^* \nabla \psi - \psi \nabla \psi^* \right) \quad (106)$$

$$\Rightarrow (\nabla \times \mathbf{v})_k = \frac{\hbar}{mi} \epsilon_{ijk} \left( (\nabla \psi^*)_i (\nabla \psi)_j - (\nabla \psi)_i (\nabla \psi^*)_j \right). \quad (107)$$

However, the state  $\psi(\mathbf{r})$  in Eq.(104) satisfies

$$(\nabla \psi^*(\mathbf{r}))_i (\nabla \psi(\mathbf{r}))_j - (\nabla \psi(\mathbf{r}))_i (\nabla \psi^*(\mathbf{r}))_j \quad (108)$$

$$= \sum_{\mathbf{k}\mathbf{k}'} k_i k'_j \left\{ \left( -\alpha_{\mathbf{k}} e^{-i\mathbf{k}\cdot\mathbf{r}} + \beta_{\mathbf{k}} e^{i\mathbf{k}\cdot\mathbf{r}} \right) \left( \alpha_{\mathbf{k}'} e^{i\mathbf{k}'\cdot\mathbf{r}} - \beta_{\mathbf{k}'} e^{-i\mathbf{k}'\cdot\mathbf{r}} \right) - \left( \alpha_{\mathbf{k}} e^{i\mathbf{k}\cdot\mathbf{r}} - \beta_{\mathbf{k}} e^{-i\mathbf{k}\cdot\mathbf{r}} \right) \left( -\alpha_{\mathbf{k}'} e^{-i\mathbf{k}'\cdot\mathbf{r}} + \beta_{\mathbf{k}'} e^{i\mathbf{k}'\cdot\mathbf{r}} \right) \right\} \quad (109)$$

$$= \sum_{\mathbf{k}\mathbf{k}'} k_i k'_j \left\{ \left( \alpha_{\mathbf{k}} e^{i\mathbf{k}\cdot\mathbf{r}} - \beta_{\mathbf{k}} e^{-i\mathbf{k}\cdot\mathbf{r}} \right) \left( -\alpha_{\mathbf{k}'} e^{-i\mathbf{k}'\cdot\mathbf{r}} + \beta_{\mathbf{k}'} e^{i\mathbf{k}'\cdot\mathbf{r}} \right) - \left( -\alpha_{\mathbf{k}} e^{-i\mathbf{k}\cdot\mathbf{r}} + \beta_{\mathbf{k}} e^{i\mathbf{k}\cdot\mathbf{r}} \right) \left( \alpha_{\mathbf{k}'} e^{i\mathbf{k}'\cdot\mathbf{r}} - \beta_{\mathbf{k}'} e^{-i\mathbf{k}'\cdot\mathbf{r}} \right) \right\} \quad (110)$$

$$= -(\nabla \psi^*(\mathbf{r}))_i (\nabla \psi(\mathbf{r}))_j - (\nabla \psi(\mathbf{r}))_i (\nabla \psi^*(\mathbf{r}))_j \quad (111)$$

$$\Rightarrow (\nabla \psi^*(\mathbf{r}))_i (\nabla \psi(\mathbf{r}))_j - (\nabla \psi(\mathbf{r}))_i (\nabla \psi^*(\mathbf{r}))_j = 0, \quad (112)$$

where the inversion symmetric coefficients  $\alpha_{-\mathbf{k}} = \alpha_{\mathbf{k}}$  and  $\beta_{-\mathbf{k}} = \beta_{\mathbf{k}}$  were used to go from the second line to the third. The curl of the flow vanishes upon inserting the wave property of Eq.(108) into the irrotational condition in Eq.(107), proving that  $\psi(\mathbf{r})$  satisfies the condition of potential flow  $\nabla \times \mathbf{v} = 0$ . Note that this proof simply verifies, under general conditions, the well-known fact that longitudinal waves, quantized or otherwise, always satisfy the condition of potential flow<sup>7</sup>.

To prove Theorem 2, it is sufficient to study the flow in a region where the boundary runs parallel to the flow direction and encloses the cross-section of the flow. In this case, the boundary condition for viscous flow, in the long-time regime where the flow is allowed to approach equilibrium with the boundary, simply becomes

$$\mathbf{v}_{\text{bdry}}(\mathbf{r}_{\text{wall}}) = \mathbf{v}_{\text{wall}}(\mathbf{r}_{\text{wall}}) = \mathbf{w}, \quad (113)$$

where  $\mathbf{v}_{\text{bdry}}$  is the flow at the boundary,  $\mathbf{v}_{\text{wall}}$  is the (inertial) motion of the boundary itself located at positions  $\mathbf{r}_{\text{wall}}$ , and  $\mathbf{w}$  is a constant independent of position along the boundary since the boundary is assumed to come from an inertial rigid body.

Irrotational flow  $\nabla \times \mathbf{v} = 0$  restricts the flow function  $\mathbf{v}(\mathbf{r})$  for this region to be only a function of the longitudinal direction

$$\mathbf{v}(\mathbf{r}) = \mathbf{v}(r_{\parallel}), \quad (114)$$

where the position vector has been separated into components parallel and perpendicular to the flow respectively  $\mathbf{r} = \mathbf{r}_{\parallel} + \mathbf{r}_{\perp}$ . On the other hand, the boundary condition in Eq.(113), coming from a rigid inertial body, further restricts the flow to a constant, independent of the longitudinal direction as well

$$\mathbf{v}(\mathbf{r}) = \mathbf{w}. \quad (115)$$

Since Eq.(105) directly relates this uniform flow  $\mathbf{v} = \mathbf{w}$  to the state  $\psi(\mathbf{r})$ , the restriction in Eq.(115) restricts the state itself. In particular, only a plane wave  $\psi(\mathbf{r}) \equiv e^{-i\mathbf{k}\cdot\mathbf{r}}$  results in a uniform flow  $\hbar\mathbf{k}/m$ .

The requirement of a plane wave state  $\psi(\mathbf{r}) \equiv e^{-i\mathbf{k}\cdot\mathbf{r}}$  in Theorem 2, requires all modes to vanish except one at  $\hbar\mathbf{k}/m = \mathbf{w}$  for the state  $\psi(\mathbf{r})$  in Eq.(104). However, the remaining mode can only satisfy this condition in a single inertial frame, since it transforms (for new frame of relative velocity change  $\mathbf{u}$  written with prime notation)  $\mathbf{k}' = \mathbf{k}$  trivially as a wave, whereas the boundary transforms as a mass  $M$  rigid body  $\mathbf{w}' = \mathbf{w} - \mathbf{u}$ . Therefore, we have also proven Corollary 1 in that the state defined in Theorem 1 cannot satisfy the conditions in Theorem 2 for an arbitrary inertial frame. Since the conditions in Theorem 2 are required for a state such as  $\psi(\mathbf{r})$  to represent the normal fluid, this proves that any such state cannot contribute to the normal fluid response.

## VII. ALTERNATIVE DERIVATION VIA STATIC RESPONSE ANALOGOUS TO STANDARD TWO-FLUID PICTURE

In the main text, the rigorous quantum equivalence between the superfluid density  $\rho_s$  and the true condensation density  $\tilde{N}_0/\mathcal{V}$  (and their  $T^3$  depletion that follows) is established via analysis of the superfluid contribution to the *dynamical* response of the system. This approach has two significant advantages over the traditional “two-fluid” hydrodynamic analysis<sup>1,9</sup>, which employs a *static* response to a wall of the pipe that drags along the normal fluid component. First, dynamic response does not require such introduction of coupling to the wall with finite velocity. More importantly, it does not require describing thermal equilibrium in the presence of flows with relative motion within the system (resulting from coupling of the normal fluid component to the wall.) As shown below, such thermal equilibrium is, in fact, non-canonical, since the system contains steady flows of different velocities and thus the probability-determining internal energy cannot be associated with the total energy of the system in any single inertial frame<sup>10</sup>.

In contrast, for dynamical susceptibilities, the thermal equilibrium is reached *before* the infinitesimal external field (that triggers the response) is introduced. This clean separation of thermal statistics from quantum dynamics grants us the strategy to first establish a *state-independent* quantum equivalence between the superfluid density  $\rho_s$  and true condensation density  $\tilde{N}_0/\mathcal{V}$ . Then, thermal statistics on the simpler true condensation density straightforwardly follows the standard Bose-Einstein distribution in the unperturbed system, whose internal energy is easily identified in the rest frame without internal relative flow.

Nonetheless, analogous to the “two-fluid” hydrodynamic analysis, one can still derive the same quantum equivalence between  $\rho_s$  and the true condensation density  $\tilde{N}_0/\mathcal{V}$  through static response to a wall of finite relative velocity. Consider a system with superfluidity flowing steadily with relative velocity  $\mathbf{v}$  along the wall of a pipe or a container. Let’s first prepare the system in its ground state [c.f. Eq.(5) of the main text] in the rest frame of the superflow, with all  $N$  particles condensing to  $\tilde{a}_0^\dagger$ , as indicated by the blue dot in Fig. 1(b). Trivially, evaluation of the normal fluid density via total momentum  $\mathbf{P}$  of the system in the rest frame,  $\rho_n = P/(\mathbf{v}\mathcal{V}) = 0$ , gives the correct result zero. Consistently in the wall frame shown in Fig. 1(a), all  $N$  particles are moving with the same velocity  $\mathbf{v}$  as part of the true condensate. Evaluation of superfluid density via  $\rho_s = P'/(\mathbf{v}\mathcal{V}) = mN/\mathcal{V} = m\tilde{N}_0/\mathcal{V}$  also produces the correct superfluid density corresponding to the true condensation density (equal to total density in this case.)

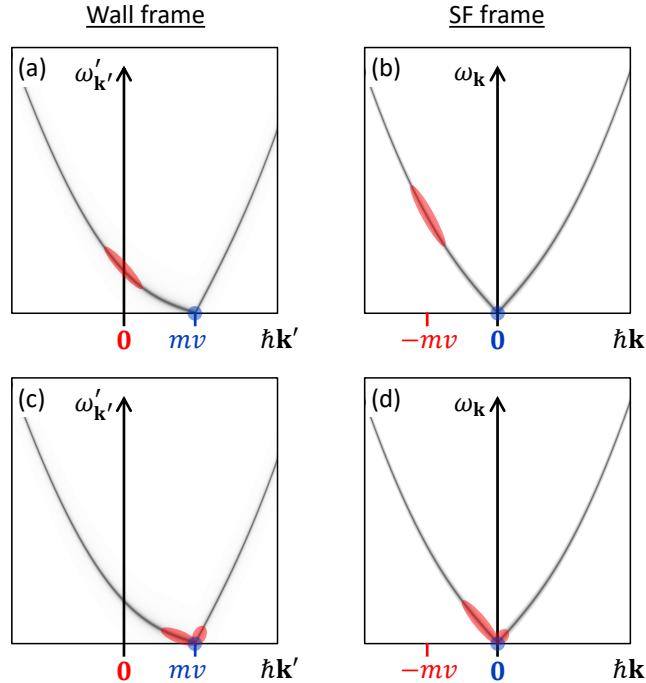

FIG. 1: Visualizing superfluid fraction upon coupling the system to an external wall with relative velocity  $\mathbf{v}$ . Notice that the dispersion relationship shown here is between the excitation energy  $\omega_{\mathbf{k}}$  and kinematic momentum  $\hbar\mathbf{k}$  of the thermally excited dressed particles, *not* the canonical momentum of the elementary particle-hole excitation (sound),  $\hbar(\mathbf{k} - \mathbf{k}_0)$ . (a) Upon reaching equilibrium with the wall, the excited dressed particles (in red) altogether appear immobile in the wall frame, and only those in the true condensate (in blue) are moving with a steady velocity  $\mathbf{v}$ . (b) Consistently, in the rest frame of the superfluid, the average velocity of the excited dressed particles (in red) is identical to the wall velocity. In contrast, standard hydrodynamic description in (c) and (d) assumes canonical population of low-energy phonons, resulting in significant underestimation of normal fluid fraction and consistently overestimating the superfluid fraction at finite temperature, and thus a slower thermal depletion.

Now, let's slowly raise the temperature to a finite value  $T$  and allow the system to reach thermal equilibrium *with* the wall. While the coupling to the wall does not affect the superfluid component owing to superflow's dissipation-less nature, it does impact the thermally-activated normal fluid component  $\tilde{a}_{\mathbf{k}}^\dagger$  of various momentum  $\mathbf{k}$ , such that on average the normal fluid component becomes *stationary* against the wall, as illustrated by the red ellipsoid in Fig. 1(a) and (b). A thermally accessible quantum pure state containing such normal fluid component is thus equivalent to a quantum gas state of "sound" modes,  $\tilde{\alpha}_{\mathbf{k}}^\dagger \equiv \tilde{a}_{\mathbf{k}}^\dagger \tilde{a}_0$ , upon interpreting the  $N$ -particle ground state as the vacuum. Note that the above *stationary* boundary condition with the wall requires that in the wall frame the total momentum of the normal fluid component in such a pure state cannot be too far from zero,  $\mathbf{P}'_n \equiv \sum_{\mathbf{k}' \neq \mathbf{0}} \hbar \mathbf{k}' \tilde{a}_{\mathbf{k}'}^\dagger \tilde{a}_{\mathbf{k}'} \sim 0$ , where  $\hbar \mathbf{0}' = m\mathbf{v}$  denotes the momentum of (blue) dressed particles in the true condensate. Therefore, evaluation of the superfluid density via  $\rho_s = P'/(v\mathcal{V}) = m\tilde{N}_0/\mathcal{V}$  produces a superfluid density equivalent to the true condensation density  $\tilde{N}_0$ . Consistently, in the superfluid rest frame the total momentum of the normal fluid component,  $\mathbf{P}_n = \mathbf{P}'_n + (1 - \tilde{N}_0)m\mathbf{v} = (1 - \tilde{N}_0)m\mathbf{v}$ , so again the normal fluid density is  $\rho_n = P/(v\mathcal{V}) = m(1 - \tilde{N}_0)/\mathcal{V}$  as expected from mass conservation. We have thus again established the quantum equivalence between the superfluid density  $\rho_s$  and the true condensate  $\tilde{N}_0/\mathcal{V}$ , through a static response to a moving wall. In particular, beyond the standard sound mode picture, our microscopic particle description allows a *strict* satisfaction of the physical boundary condition associated with equilibrium with the moving wall.

Crucially, the microscopic particle picture also reveals an important *non-canonical* nature of the thermal equilibrium involving a moving wall. Indeed, notice that the occupation distribution in Fig. 1(a) and (b) has a gap at low energy and thus clearly cannot possibly correspond to the standard Bose-Einstein distribution. The physical origin of such finite energy requirement is associated with the finite velocity of the wall in the superflow's rest frame. During the slow increase of temperature from zero, consider a newly thermally enabled low-energy excited pure state corresponding to promoting one dressed particle from the true condensate to one with nearly the same zero momentum. Coupling to the wall would attempt to drag this dressed particle along the wall, which in turn would slow down the wall to conserve the total momentum of the system. To maintain the assigned fixed velocity of the wall, external supply of additional energy to the system is thus necessary, until the dressed particle finally catches up with the wall and reaches the physical thermal equilibrium. The total energy injected into the system is, of course, exactly the energy required to accelerate the excited particle from nearly stationary up to the constant velocity of the wall in this superflow rest frame.

The above non-canonical thermal statistics, therefore, qualitatively differs from that employed in the traditional hydrodynamic two-fluid picture. As illustrated in Fig. 1(c), the excitations are traditionally assumed to be thermally populated sound modes,  $\tilde{a}_{\mathbf{k}}^\dagger \tilde{a}_0$ , following the canonical Boltzmann distribution and to have zero average *group velocity* in the wall frame<sup>8,9</sup>. Correspondingly, in the superflow rest frame the Bose-Einstein distribution function takes the form<sup>9</sup>  $n_B(\omega_{\mathbf{k}} + \hbar \mathbf{k} \cdot \mathbf{v})$  according to the boosted excitation energy  $\omega_{\mathbf{k}}$  and dressed particle momentum  $\mathbf{k}$ . Note, however, that such distribution would give the excited dressed particles an average velocity  $\hbar \mathbf{k}/m$  only slightly deviating from that of the superflow. In other words, instead of sticking to the wall, at equilibrium the dressed particles would still *unphysically* follow the superflow, even in the absence of friction between the normal and superfluid components.

Naturally, in such a physically inconsistent thermal distribution, estimation of the normal fluid density via total momentum  $\mathbf{P}$  in the superfluid rest frame,  $\rho_n = P/(v\mathcal{V}) \ll m(1 - \tilde{N}_0)/\mathcal{V}$ , would result in a significantly smaller normal fluid density, since as illustrated in Fig. 1(d) the total kinematic momentum of the system is much smaller than  $m\mathbf{v}(1 - \tilde{N}_0)$ . Similarly, a much larger superfluid density would result from  $\rho_s = P'/(v\mathcal{V}) \gg m\tilde{N}_0/\mathcal{V}$ , since the total momentum  $\mathbf{P}'$  of the system in the wall frame shown in Fig. 1(c) incorrectly includes dissipative normal contributions from the excited particles (in red) as well.

Such difference in statistical treatments leads to distinct results on the thermal fluctuation of superfluid density. In the linear response regime  $\mathbf{v} \rightarrow \mathbf{0}$ , our superfluid fraction is simply the complement of the thermal population of normal fluid density  $\langle \tilde{N}_0 \rangle/N = 1 - \langle \sum_{\mathbf{k} \neq \mathbf{0}} \tilde{a}_{\mathbf{k}}^\dagger \tilde{a}_{\mathbf{k}} \rangle/N$ , which gives a  $T^3$  thermal depletion for a linear energy-momentum dispersion of the sound modes. The above overestimation of finite-temperature superfluid density in canonical statistics, on the other hand, leads to a slower  $T^4$  depletion instead.

In essence, the use of dynamical response in the main text circumvents the complications of non-canonical statistics associated with the presence of steady relative flows within the system. Upon first establishing the rigorous quantum equivalence between the superfluid density and the true condensation density, thermal fluctuations of the former can be straightforwardly evaluated through the canonical thermal occupation of the latter without invoking non-canonical statistics associated with equilibrium with a moving wall. This section demonstrates that this essential quantum equivalence can also be established via static response analogous to the two-fluid picture, *as long as* the physical boundary condition required by equilibrium with a moving wall is strictly satisfied. Our resulting  $T^3$  thermal depletion of superfluid density consequently differs from the traditional lore due to our 'proper' handling of the non-canonical statistics.

### VIII. EFFECTS OF WEAK IMPURITIES AT LOW TEMPERATURE

In this final section we briefly outline the dominant low-temperature effect of local impurities on the superfluid density. For simplicity, we introduce local impurities via a local random on-site potential

$$H_{\text{dis}} = \sum_{\mathbf{x}} \delta(\mathbf{x}) a_{\mathbf{x}}^{\dagger} a_{\mathbf{x}} \quad (116)$$

$$\delta \in \frac{1}{\sqrt{2\pi\Delta}} e^{-\frac{y^2}{2\Delta}} \quad y \in \{-\infty, \infty\}, \quad (117)$$

where  $\delta(\mathbf{x})$  instances a Gaussian random variable taken from the probability density function  $\delta$  at each point  $\mathbf{x}$ . WLOG we have fixed the average to vanish, leaving the variance  $\Delta$  as the only remaining disorder scale

$$\bar{\delta} = 0 \quad (118)$$

$$\overline{\delta^2} \equiv \Delta \ll 1, \quad (119)$$

and therefore we perform a perturbative expansion in weak disorder  $\Delta \ll 1$  to identify the qualitative effects of impurities on superfluidity.

Throughout the rest of this section, we study the large-system limit where the effects of finite-size sampling of  $\delta$  are negligible. This is particularly easy to see for the low-energy, long-wavelength states relevant to this low-temperature study of superfluid and normal fluid responses. For example, the average effect of disorder on long-wavelength states  $|\mathbf{k}| \ll 1$  in the large system limit identifies with the population average of  $\delta$

$$\lim_{V \rightarrow \infty} \frac{1}{V} \sum_{\mathbf{x}} \delta(\mathbf{x}) e^{i\mathbf{k} \cdot \mathbf{x}} = \bar{\delta} = 0, \quad (120)$$

which vanishes. Given a system of length  $L$  and volume  $V = L^d$ , one way to show this is by coarse-graining the system into  $M \propto L^{d-1}$  arbitrarily large regions of volume  $m \propto L$ , where  $(mM) \propto V$  correctly scales with the system volume. In the large-system limit and for a sufficiently slow-varying phase mode (e.g.  $|\mathbf{k}| \propto L^{-\alpha}$  and  $1/2 < \alpha < 1$ ) we find

$$\lim_{V \rightarrow \infty} \frac{1}{V} \sum_{\mathbf{x}} \delta(\mathbf{x}) e^{i\mathbf{k} \cdot \mathbf{x}} = \lim_{V \rightarrow \infty} \frac{1}{M} \sum_{\mathbf{X}} e^{i\mathbf{k} \cdot \mathbf{X}} \left\{ \frac{1}{m} \sum_{\mathbf{x}'} \delta(\mathbf{x}') e^{i\mathbf{k} \cdot \mathbf{x}'} \right\} \quad (121)$$

$$= \lim_{V \rightarrow \infty} \frac{1}{M} \sum_{\mathbf{X}} e^{i\mathbf{k} \cdot \mathbf{X}} \left\{ \frac{1}{m} \sum_{\mathbf{x}'} \delta(\mathbf{x}') (1 + i\mathbf{k} \cdot \mathbf{x}' + \dots) \right\} \quad (122)$$

$$\leq \lim_{V \rightarrow \infty} \frac{1}{M} \sum_{\mathbf{X}} e^{i\mathbf{k} \cdot \mathbf{X}} \left\{ \frac{1}{m} \sum_{\mathbf{x}'} \delta(\mathbf{x}') (1 + im|\mathbf{k}| + \dots) \right\} \quad (123)$$

$$= \lim_{V \rightarrow \infty} \frac{1}{M} \sum_{\mathbf{X}} e^{i\mathbf{k} \cdot \mathbf{X}} \left\{ \frac{1}{M} \sum_{\mathbf{x}} \delta(\mathbf{x}) (1 + \mathcal{O}[L^{1-\alpha}]) \right\} = \lim_{V \rightarrow \infty} \bar{\delta} \left( \frac{1}{M} \sum_{\mathbf{X}} e^{i\mathbf{k} \cdot \mathbf{X}} \right) \rightarrow 0, \quad (124)$$

where our choice of exponent  $\alpha$  implies the required  $1 - \alpha > 0$  and ensures that  $\mathbf{k} \cdot \mathbf{x} \ll 2\pi$  in order to safely truncate the Taylor expansion of the phase factor. The above statistics in Eqs.(120) help identify the leading-order relevant effects of the perturbation. The first order correction to the energy vanishes

$$E_{\mathbf{k}}^{(1)} = \left\langle \psi_{\mathbf{k}}^{(0)} \left| H_{\text{dis}} \right| \psi_{\mathbf{k}}^{(0)} \right\rangle = \frac{1}{V} \sum_{\mathbf{x}} \delta(\mathbf{x}) \rightarrow 0, \quad (125)$$

where we have used the fact that  $a_{\mathbf{x}}^{\dagger} a_{\mathbf{x}} \equiv n_{\mathbf{x}} = 1/V$  for all states in the clean system (due to translation invariance).

We note that the second-order correction to the energy  $E_{\mathbf{k}}^{(2)}$ , although non-vanishing, does not contribute to the low-energy superfluid or normal fluid response in this system. This is because the low-energy spectrum of the clean system ( $\Omega_{\mathbf{k}} = v|\mathbf{k}|$ ) is linear and therefore the density of states is linear in 3D. The second-order correction to the energy merely reshuffles the density of states in a small energy window  $\Delta\omega$  around each energy  $\omega$  in proportion to the local density of states in that window. But since the density of states is linear in this region this reshuffling affects each energy in exactly the same way, resulting in no net effect.

It turns out that the first-order perturbative correction to the states *does* affect the superfluid and normal fluid densities, which are now clearly the dominant effect of weak impurities on the superfluid and normal fluid responses since neither the first- nor the second-order corrections to the energy affect these quantities.

The first order corrections to the states can be identified by computing the modification of the excitation operators  $\tilde{\alpha}_{\mathbf{k}}$  in Eq.(25) while leaving their corresponding commutators unchanged. (Generally, a truncated perturbation expansion applies a non-unitary transformation and will not preserve the commutation relations, but the resulting error is controlled by the smallness of the perturbation parameter. In this case the small variance  $\Delta \ll 1$  as well as the long-wavelength  $|\mathbf{k}| \ll 1$  assumption make this error negligible). Since the unperturbed system in Eq.(25) is diagonal in  $\tilde{\alpha}_{\mathbf{k}}$ , the first order perturbative corrections to the state

$$c_{\mathbf{k}\mathbf{k}'}^{(1)} = \frac{\langle \psi_{\mathbf{k}'} | H_{\text{dis}} | \psi_{\mathbf{k}} | \psi_{\mathbf{k}'} | H_{\text{dis}} | \psi_{\mathbf{k}} \rangle}{E_{\mathbf{k}}^{(0)} - E_{\mathbf{k}'}^{(0)}} \quad (126)$$

can be represented by the corresponding corrections to the one-body operators  $\tilde{\alpha}_{\mathbf{k}}$  and  $\tilde{a}_0$ . To leading order (in  $\tilde{n}_0$ ), these terms are given by

$$\tilde{a}_0 \rightarrow \tilde{a}_0 - \sum_{\mathbf{k} \neq 0} \frac{\delta_{\mathbf{k},0}}{\Omega_{\mathbf{k}}} \left( c_{\mathbf{k}} \tilde{\alpha}_{\mathbf{k}} - d_{\mathbf{k}} b \tilde{\alpha}_{-\mathbf{k}}^\dagger \right) \quad (127)$$

$$\tilde{a}_0^\dagger \rightarrow \tilde{a}_0^\dagger + \sum_{\mathbf{k} \neq 0} \frac{\delta_{\mathbf{k},0}}{\Omega_{\mathbf{k}}} \left( c_{\mathbf{k}} \tilde{\alpha}_{\mathbf{k}}^\dagger - d_{\mathbf{k}} \tilde{\alpha}_{-\mathbf{k}} \right) \quad (128)$$

$$\tilde{\alpha}_{\mathbf{k}} \rightarrow \tilde{\alpha}_{\mathbf{k}} + \frac{\delta_{\mathbf{k},0}}{\Omega_{\mathbf{k}}} \left( c_{\mathbf{k}} \tilde{\alpha}_{\mathbf{k}} - d_{\mathbf{k}} \tilde{\alpha}_{-\mathbf{k}}^\dagger \right) \quad (129)$$

$$\tilde{\alpha}_{\mathbf{k}}^\dagger \rightarrow \tilde{\alpha}_{\mathbf{k}}^\dagger - \frac{\delta_{\mathbf{k},0}}{\Omega_{\mathbf{k}}} \left( c_{\mathbf{k}} \tilde{\alpha}_{\mathbf{k}}^\dagger - d_{\mathbf{k}} \tilde{\alpha}_{-\mathbf{k}} \right). \quad (130)$$

Since the current operator is independent of any local density term in the Hamiltonian, including the weak impurity term in Eq.(116), the formal derivation of the normal fluid and superfluid densities, given in Eqs.(??,??) respectively, remains unaffected by the introduction of the weak impurity term. Applying the perturbation identified in Eqs.(127-130) to these fluid response equations

$$\rho_s = m(\tilde{n}_0 - n^{(1)}) \quad (131)$$

$$\rho_n = m(n - \tilde{n}_0 + n^{(1)}) \quad (132)$$

$$n^{(1)} \equiv \frac{1}{m} \sum_{\mathbf{k} \neq 0} \frac{\delta_{\mathbf{k},0}^2}{\Omega_{\mathbf{k}}^2} \left\langle \tilde{\alpha}_{\mathbf{k}}^\dagger \tilde{\alpha}_{\mathbf{k}} \middle| \tilde{\alpha}_{\mathbf{k}}^\dagger \tilde{\alpha}_{\mathbf{k}} \right\rangle \approx \left( \frac{\Delta k_B}{4\pi^2 U \tilde{n}_0 c} \log(t) \right) T \quad (133)$$

results in a dominant low-temperature  $T$ -linear reduction in the superfluid density and corresponding growth of the normal fluid density as per the sum rule.

The above result shows that the leading order effect of weak impurities with temperature is to reduce the superfluid density linearly  $\propto T$ , which is a much stronger reduction than the  $\propto T^3$  reduction found for the clean case in section IV, as expected. Further, the result of this leading order perturbation is consistent the sum rule, since the normal fluid density also increases linearly  $\propto T$  and exactly matches the reduction of the superfluid density.

## IX. FITTING PROCEDURE FOR THE EXPERIMENTAL DATA COLLAPSE

In this section we describe the procedure used to generate the data collapse plots in Figure 1 of the main text. For clarity, we illustrate the procedure for LaNiGa<sub>2</sub> as an example. A figure taken from<sup>11</sup> is displayed in Fig. 2(a). Using the Origin Digitizer, we extract the superfluid density data displayed in Fig. 2(b) and fit the extracted data to a single power-law curve of the form

$$\rho_s(T)/\rho_s(0) = 1 - AT^\gamma. \quad (134)$$

Since we are interested in the low-temperature behavior of the superfluid density in these materials, we discard data near the transition temperature systematically until we find that the fitting procedure appears to converge. The result of such a converged fitting is displayed as a red dotted line in Fig. 2(b). In fact, all of the materials presented here exhibit a resulting power-law fitting with  $\gamma \sim 3$ , and to illustrate this fact we present three such fittings side-by-side in Fig. 3.

We are interested in the leading order fluctuations at the lowest temperatures and far from any phase transition. A cursory attempt to fit to a (gapped) exponential indicates it is an extremely poor fit, so we search for integer power-law monomial behavior. To that end, we simply display each data set along with best fit lines for fixed integer exponents ( $\gamma = 2, 3, 4$  corresponding to purple, red, and blue dotted lines respectively) in Fig. 2(c), where it is clear that  $\gamma = 2$  and  $\gamma = 4$  each provide very poor fits that

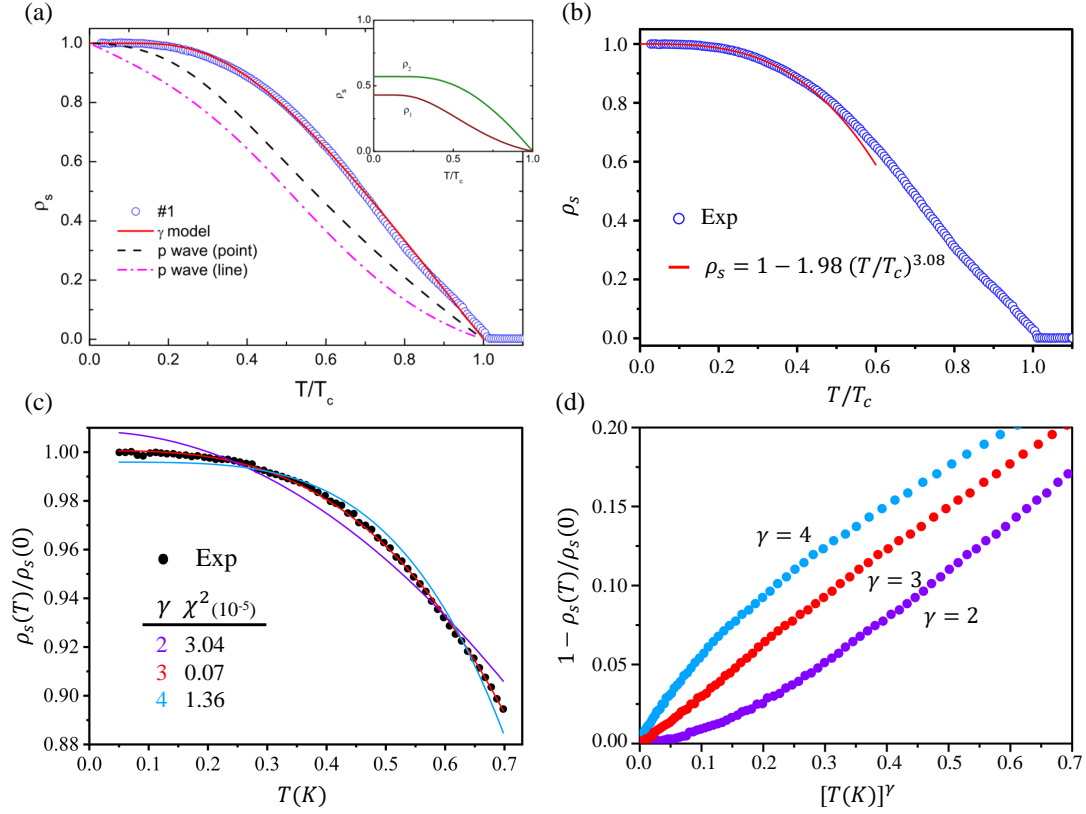

FIG. 2: Fitting procedure applied to (a) the superfluid density  $\rho_s$  vs reduced temperature  $T/T_c$  in a data set<sup>11</sup> for LaNiGa<sub>2</sub>. (b) Extracted data (blue) from (a) with best-fit power-law line (red) fit to data below a threshold where the fit converges. (c) A simple comparison between power-law least squares fitting with exponents  $\gamma = 2, 3, 4$  (purple, red, blue) of the data set in (b). Notice that the  $\gamma = 2$  and  $\gamma = 4$  fit very poorly with opposite data clustering above and below the fit line, indicating that the best fit lies between them. (d) Plot of  $1 - \rho_s$  vs  $T^\gamma$  clearly illustrating that  $\gamma = 3$  fits very well (i.e. converges to a straight line) at low temperature, unlike  $\gamma = 2$  or  $\gamma = 4$ .

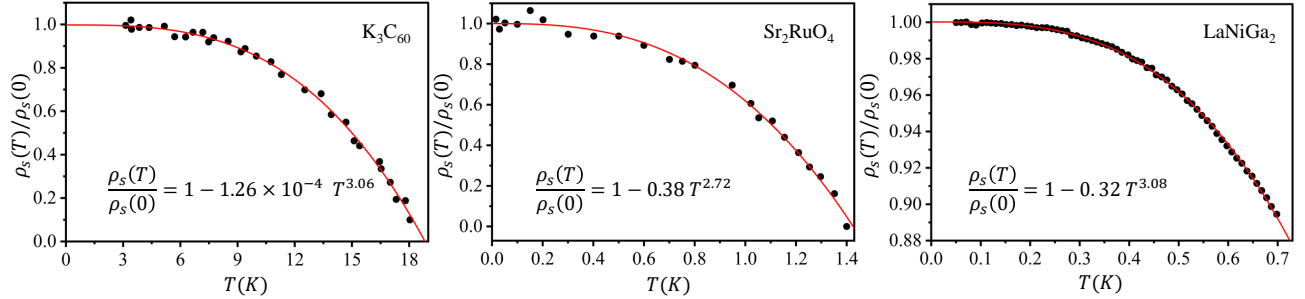

FIG. 3: Comparison similar to Fig. 2(c) above for three data sets<sup>11–13</sup> presented in the main text. Notice that  $\gamma \sim 3$  for all of them.

significantly underestimate and overestimate  $\gamma$  respectively. To see the convergence to  $\gamma = 3$  more clearly in this example, we plot  $1 - \rho_s(T)/\rho_s(0)$  vs  $T^\gamma$  in Fig. 2(d) to show that the data converge to a straight line (red points) for  $\gamma = 3$  but not for  $\gamma = 2$  (purple) or  $\gamma = 4$  (blue). In Fig. 4 we display the integer exponent fitting, analogous to Fig. 2(c), for each data set presented in the main text.

In order to display the results in a single data-collapse figure, especially since the onset temperature of this effect ( $\sim 0.14\text{K} - 18.05\text{K}$ ) spans more than two orders of magnitude across all of these materials, we further rescale the temperature to absorb the coefficient

$$\tilde{T} = A^{-\frac{1}{3}}. \quad (135)$$

Finally, in the inset of Figure 1 in the main text, we illustrate the convergence of all data sets to  $\gamma = 3$  via a plot analogous to

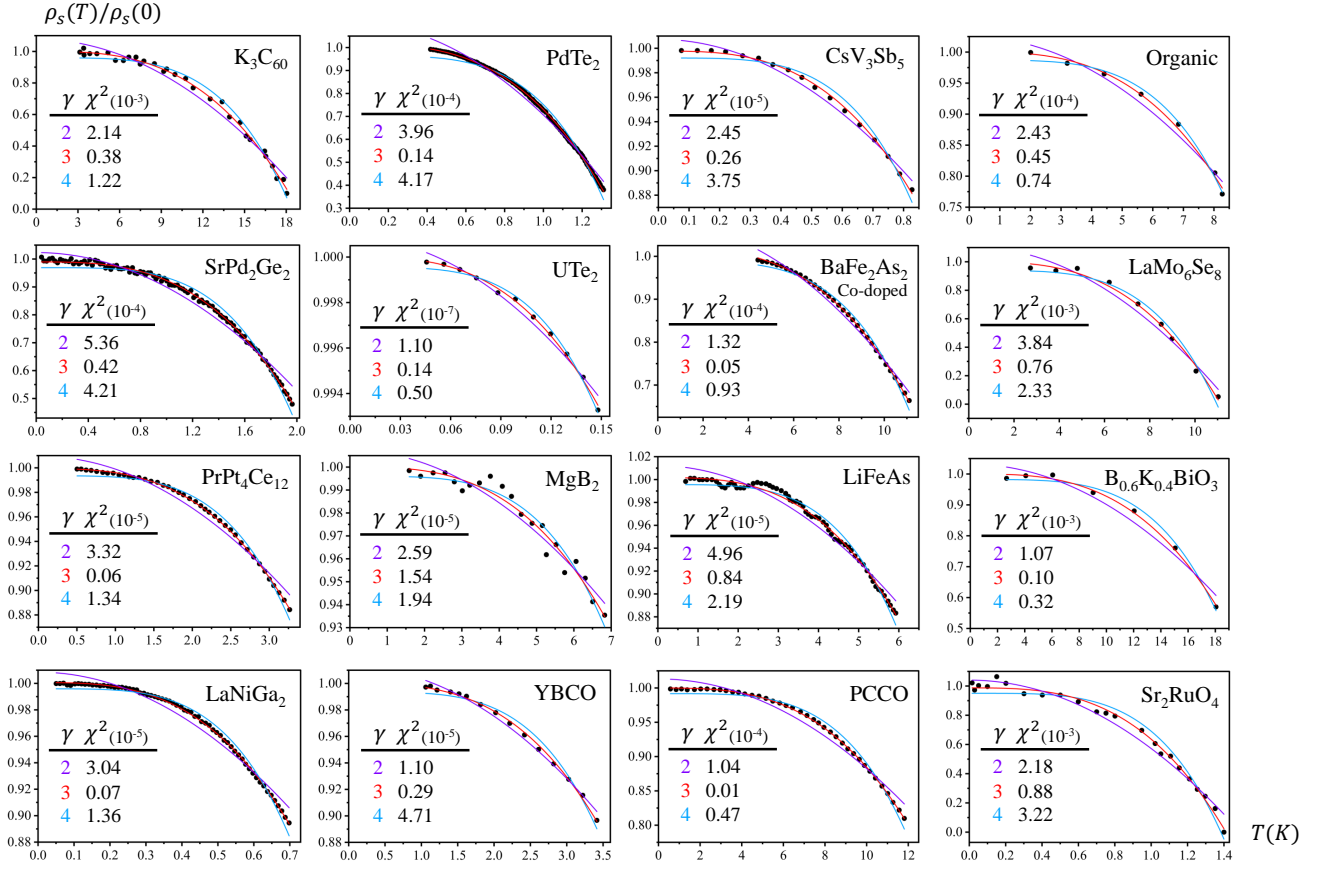

FIG. 4: Least squares fitting to a power-law monomial for several example data sets at low temperature. Note that the exponent  $\gamma \sim 3$  for each example. Chi-squared test statistic values are displayed for each fit, indicating that  $\gamma = 3$  is the best fit among them by significant margin in all cases presented here.

the example in Fig. 2(d). For clarity, we introduce a data-set dependent ‘zoom’ factor  $Z$ , identified for each material in Table I, such that the deviation from  $\gamma = 3$  occurs at around the same point in the inset.

TABLE I: Inverse of zoom factor  $1/Z$  for different materials in Figure 1.

| Material                                                                            | $1/Z$ |
|-------------------------------------------------------------------------------------|-------|
| MgB <sub>2</sub> <sup>14</sup>                                                      | 0.07  |
| CsV <sub>3</sub> Sb <sub>5</sub> <sup>15</sup>                                      | 0.15  |
| LiFeAs <sup>16</sup>                                                                | 0.13  |
| NbSe <sub>2</sub> <sup>17</sup>                                                     | 0.1   |
| LaNiGa <sub>2</sub> <sup>11</sup>                                                   | 0.25  |
| Ba(Fe <sub>0.9</sub> Co <sub>0.1</sub> ) <sub>2</sub> As <sub>2</sub> <sup>18</sup> | 0.35  |
| PrPt <sub>4</sub> Ge <sub>12</sub> <sup>19</sup>                                    | 0.18  |
| PdTe <sub>2</sub> <sup>20</sup>                                                     | 0.6   |
| K <sub>3</sub> C <sub>60</sub> <sup>12</sup>                                        | 1     |
| SrPd <sub>2</sub> Ge <sub>2</sub> <sup>21</sup>                                     | 0.5   |
| Sr <sub>0.9</sub> La <sub>0.1</sub> CuO <sub>2</sub> <sup>22</sup>                  | 0.45  |
| Pr <sub>2-x</sub> Ce <sub>x</sub> CuO <sub>4-δ</sub> ( $x = 0.131$ ) <sup>23</sup>  | 0.08  |
| Ba <sub>0.6</sub> K <sub>0.4</sub> BiO <sub>3</sub> <sup>24</sup>                   | 0.45  |
| LaMo <sub>6</sub> Se <sub>8</sub> <sup>25</sup>                                     | 0.45  |
| Sr <sub>2</sub> RuO <sub>4</sub> <sup>13</sup>                                      | 0.7   |
| UTe <sub>2</sub> <sup>26</sup>                                                      | 0.015 |
| $\kappa$ -(BEDT-TTF) <sub>2</sub> Cu[N(CN) <sub>2</sub> ]Br <sup>27</sup>           | 0.2   |

## X. DOPING-INDEPENDENT UNIVERSAL LOW-TEMPERATURE SUPERFLUID DENSITY DEPLETION IN YBCO

In this section we study the low-temperature superfluid density in underdoped YBa<sub>2</sub>Cu<sub>3</sub>O<sub>6+δ</sub> measurements<sup>28</sup> over a range of doping. As illustrated in Fig.5(a), this relatively high-quality sample exhibits  $T^3$  depletion of the superfluid density  $\rho_s \propto 1/\lambda^2$  via the penetration depth  $\lambda$  over the entire doping range of the study. In Fig.5(b) we perform the same data collapse as in Figure 1 of the main text and described in detail in section XI of the appendix, fit to the function in Eq.(134) to clearly display the universal depletion of the superfluid density at low temperature  $\rho_s(T)/\rho_s(0) = 1 - (T/\tilde{T})^3$ , where  $\tilde{T}$  is defined in Eq.(135).

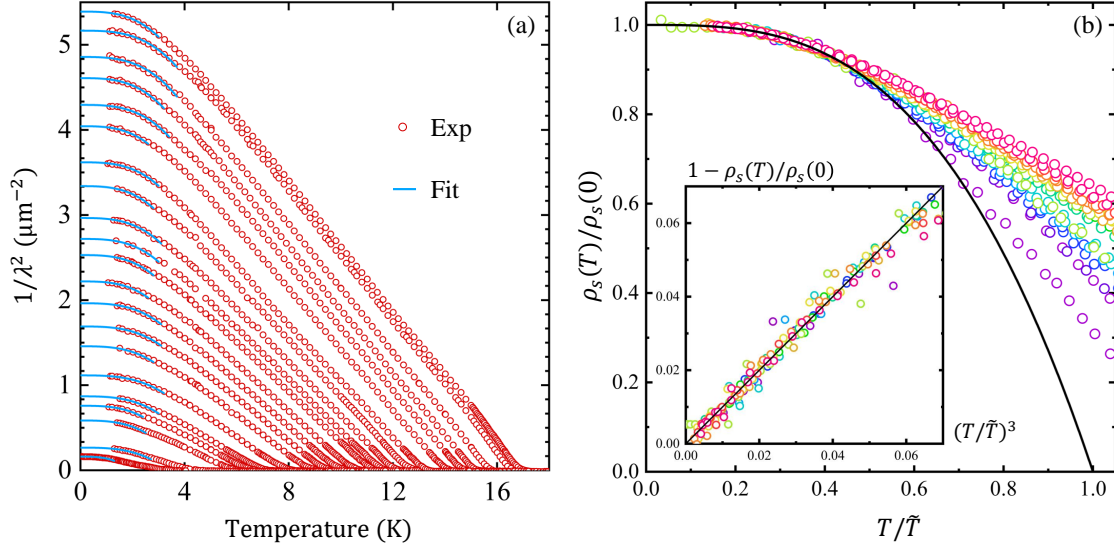

FIG. 5: (a) Superfluid density via penetration depth measurements  $\rho_s \propto 1/\lambda^2$  in YBa<sub>2</sub>Cu<sub>3</sub>O<sub>6+δ</sub><sup>28</sup> showing  $T^3$  depletion indicated in blue. (b) Collapse of the data in (a) to a single universal  $1 - (T/\tilde{T})^3$  curve as a function of rescaled temperature  $T/\tilde{T}$ . The inset in (b), similar to Figure 1 in the main text, shows that  $T^3$  remains a good fit down to the lowest temperatures of the study.

- <sup>1</sup> in *Collected Papers of L.D. Landau*, edited by D. Ter Haar (Pergamon, 1965), pp. 301–330, ISBN 978-0-08-010586-4.
- <sup>2</sup> P. W. Anderson, *Phys. rev.* **86** (1952).
- <sup>3</sup> G. D. Mahan, *Many-Particle Physics* (Plenum, New York, 2000), 3rd ed.
- <sup>4</sup> L. P. Kadanoff, , and P. C. Martin, *Annals of Physics* **24**, 419 (1963).
- <sup>5</sup> J. W. Negele and H. Orland, *Quantum Many-Particle Systems* (Westview Press, 1998).
- <sup>6</sup> I. Fujiwara, D. ter Haar, and H. Wergeland, *Journal of Statistical Physics* **2**, 329 (1970).
- <sup>7</sup> L. Landau, *Physical Review* **60** (1941).
- <sup>8</sup> B. V. Svistunov, E. S. Babaev, and N. V. Prokof'ev, *Superfluid states of matter* (Crc Press, 2015).
- <sup>9</sup> L. D. Landau and E. M. Lifshitz, *Statistical Physics*, vol. 3 (Pergamon Press Ltd., London-Paris, 1958).
- <sup>10</sup> W. Ku and A. Hegg, arXiv e-prints arXiv:2401.08576 (2024), URL <https://arxiv.org/abs/2401.08576>.
- <sup>11</sup> Z. F. Weng, J. L. Zhang, M. Smidman, T. Shang, J. Quintanilla, J. F. Annett, M. Nicklas, G. M. Pang, L. Jiao, W. B. Jiang, et al., *Phys. Rev. Lett.* **117**, 027001 (2016), URL <https://link.aps.org/doi/10.1103/PhysRevLett.117.027001>.
- <sup>12</sup> Y. J. Uemura, A. Keren, L. P. Le, G. M. Luke, W. D. Wu, J. S. Tsai, K. Tanigaki, K. Holczer, S. Donovan, and R. L. Whetten, *Physica C Superconductivity* **235**, 2501 (1994).
- <sup>13</sup> R. Khasanov, A. Ramires, V. Grinenko, I. Shipulin, N. Kikugawa, D. A. Sokolov, J. A. Krieger, T. J. Hicken, Y. Maeno, H. Luetkens, et al., *Phys. Rev. Lett.* **131**, 236001 (2023), URL <https://link.aps.org/doi/10.1103/PhysRevLett.131.236001>.
- <sup>14</sup> H. Kim, K. Cho, M. A. Tanatar, V. Taufour, S. K. Kim, S. L. Bud'ko, P. C. Canfield, V. G. Kogan, and R. Prozorov, *Symmetry* **11** (2019), ISSN 2073-8994, URL <https://www.mdpi.com/2073-8994/11/8/1012>.
- <sup>15</sup> W. Duan, Z. Nie, S. Luo, F. Yu, B. R. Ortiz, L. Yin, H. Su, F. Du, A. Wang, Y. Chen, et al., *Science China Physics, Mechanics & Astronomy* **64** (2021), URL <https://doi.org/10.1007/s11433-021-1747-7>.
- <sup>16</sup> H. Kim, M. A. Tanatar, Y. J. Song, Y. S. Kwon, and R. Prozorov, *Phys. Rev. B* **83**, 100502 (2011), URL <https://link.aps.org/doi/10.1103/PhysRevB.83.100502>.
- <sup>17</sup> J. D. Fletcher, A. Carrington, P. Diener, P. Rodière, J. P. Brison, R. Prozorov, T. Olheiser, and R. W. Giannetta, *Phys. Rev. Lett.* **98**, 057003 (2007), URL <https://link.aps.org/doi/10.1103/PhysRevLett.98.057003>.
- <sup>18</sup> A. Karakozov, S. Zapf, B. Gorshunov, Y. Ponomarev, M. Magnitskaya, E. Zhukova, A. Prokhorov, V. Anzin, and S. Haindl, *Physical Review B* **90** (2014).
- <sup>19</sup> J. L. Zhang, Y. Chen, L. Jiao, R. Gumenuik, M. Nicklas, Y. H. Chen, L. Yang, B. H. Fu, W. Schnelle, H. Rosner, et al., *Phys. Rev. B* **87**, 064502 (2013), URL <https://link.aps.org/doi/10.1103/PhysRevB.87.064502>.
- <sup>20</sup> M. V. Salis, P. Rodière, H. Leng, Y. K. Huang, and A. de Visser, *Journal of Physics: Condensed Matter* **30**, 505602 (2018).
- <sup>21</sup> H. Kim, N. H. Sung, B. K. Cho, M. A. Tanatar, and R. Prozorov, *Phys. Rev. B* **87**, 094515 (2013), URL <https://link.aps.org/doi/10.1103/PhysRevB.87.094515>.
- <sup>22</sup> R. Khasanov, A. Shengelaya, R. Brutsch, and H. Keller, *Condensed Matter* **5** (2020), URL <https://www.mdpi.com/2410-3896/5/3/50>.
- <sup>23</sup> M.-S. Kim, J. A. Skinta, T. R. Lemberger, A. Tsukada, and M. Naito, *Phys. Rev. Lett.* **91**, 087001 (2003), URL <https://link.aps.org/doi/10.1103/PhysRevLett.91.087001>.
- <sup>24</sup> Y. J. Uemura, L. P. Le, G. M. Luke, B. J. Sternlieb, W. D. Wu, J. H. Brewer, T. M. Riseman, C. L. Seaman, M. B. Maple, M. Ishikawa, et al., *Phys. Rev. Lett.* **66**, 2665 (1991), URL <https://link.aps.org/doi/10.1103/PhysRevLett.66.2665>.
- <sup>25</sup> T. Shang, W. Xie, D. J. Gawryluk, R. Khasanov, J. Z. Zhao, M. Medarde, M. Shi, H. Q. Yuan, E. Pomjakushina, and T. Shiroka, *New Journal of Physics* **22**, 093016 (2020), URL <https://dx.doi.org/10.1088/1367-2630/abac3b>.
- <sup>26</sup> K. Ishihara, M. Roppongi, M. Kobayashi, K. Imamura, Y. Mizukami, H. Sakai, P. Opletal, Y. Tokiwa, Y. Haga, K. Hashimoto, et al., *Nature Communications* **14** (2023).
- <sup>27</sup> Y. Ait Ahmed, A. Tirbiyine, D. Soubane, A. Taoufik, H. El Ouaddi, H. El hamidi, A. Abou Alhassan, A. Hafid, and S. Senoussi, *Materials Today: Proceedings* **24**, 100 (2020), ISSN 2214-7853, international Conference on Plasma and Energy Materials ICPEM2019, URL <https://www.sciencedirect.com/science/article/pii/S2214785319328834>.
- <sup>28</sup> D. M. Broun, W. A. Huttema, P. J. Turner, S. Özcan, B. Morgan, R. Liang, W. N. Hardy, and D. A. Bonn, *Phys. Rev. Lett.* **99**, 237003 (2007), URL <https://link.aps.org/doi/10.1103/PhysRevLett.99.237003>.
